# Supplementary material for: Diffusion Facial Forgery Detection
Source: arXiv:2401.15859 source file (2024-01-29)
Supplement: Supplementary file 1 [file X_suppl.tex]

\clearpage
\setcounter{page}{1}

\stepcounter{section} % 让section计数器增加1
\setcounter{section}{0} % 将section计数器重置为0
\setcounter{equation}{0}

\setcounter{figure}{0}

\setcounter{table}{0}

\setcounter{footnote}{0}
\maketitlesupplementary

\section{Abstract}
The content of this supplementary material is divided into three main sections. \Cref{supsec:Diff_Approach} provides a detailed description of the thirteen synthetic methods we employed. \Cref{supsec:Benchmarks} offers additional evaluation results, along with tables for the values in \Cref{fig:subset} and \Cref{fig:linear_probing_fintune} presented in the main manuscipt. \Cref{supsec:Visualizations} presents comprehensive visualizations, including an overview of the overall pipeline for generating forged images, as well as numerous non-cherry-picked samples from the thirteen methods.

\section{Diffusion Approaches}
\label{supsec:Diff_Approach}
We have employed a total of 13 approaches\footnote{Adjustments to the watermark implementation in released models are made to prevent detectors from discerning authenticity via watermarks.} to generate forged images, and a detailed description of these methods is as follows,
\subsection{Text-to-Image}
\begin{itemize}
    \item \textbf{Midjourney}~\cite{Midjourney} is one of the largest online-accessible AI art creation service providers. We directly invoke the `\emph{/imagine}' command to generate images from prompts.
    \item \textbf{Stable Diffusion XL (SDXL)}~\cite{SDXL}. SDXL is the drastically improved version of stable diffusion models~\cite{SD-Latent-Diffusion}, which encompasses three times of the UNet parameters of the previous ones. We utilize the official open-source code and parameters to generate images.
    \item \textbf{FreeDoM\_T}~\cite{FreeDoM} uses off-the-shelf pre-trained models to construct the energy function~\cite{Energy} and generates images with various conditions. In the T2I subset, we utilize CLIP~\cite{CLIP} as the text encoder to guide face synthesis.
    \item \textbf{HPS}~\cite{align_sd} trains a human preference classifier with the collected dataset and derive a human preference score to adapt Stable Diffusion to better align with human preferences through a human preference classifier.
\end{itemize}

% \footnote{\url{https://www.midjourney.com}.}
% \footnote{\url{https://github.com/Stability-AI}.}
% \footnote{\url{https://github.com/vvictoryuki/FreeDoM}.}
% \footnote{\url{https://github.com/tgxs002/align_sd}.}

\subsection{Image-to-Image}
\begin{itemize}
    \item \textbf{Low-Rank Adaption (LoRA) Diffusion}~\cite{LORA}. LoRA is to freeze the pre-trained model weights and inject trainable layer into the Transformer architecture, greatly reducing the number of trainable parameters for downstream tasks. With the I2I setting, we train the LoRA layer with images of one specific identity, which enables the model to learn the appearance of that identity, and output faces visually align closely with this person.
    \item \textbf{DreamBooth}~\cite{DreamBooth}.  DreamBooth offers another fine-tuning manner to personalize existing diffusion models such that it learns to bind a unique identifier to specific subject, by leveraging the semantic prior embedded with a new autogenous class-specific prior preservation loss.
    \item \textbf{SDXL Refiner}~\cite{SDXL}. The refiner model is designed to denoise the small noise of T2I-generated images from SDXL~\cite{SDEdit}, making them smoother and more realistic. 
    \item \textbf{FreeDoM\_I}. It is flexible to run FreeDoM with visual conditions. As a result, we utilize the real image with its corresponding facial appearance, sketches, landmarks, and segmentations for I2I generation. 
\end{itemize}

\subsection{Face Swapping}
\begin{itemize}
    \item \textbf{DiffFace}~\cite{DiffFace} is one of the first efforts to apply diffusion model in face swapping task, which utilizes the facial expert models to transfer source identity while preserving target attributes faithfully.
    \item \textbf{DCFace}~\cite{DCFace} combines the source and target as two conditions, \ie, appearance (ID) and external factor (style), respectively. These two conditions provide guidance to the dual-condition diffusion model and produce face images of the same subject under different styles.
\end{itemize}

\subsection{Face Editing}
\begin{itemize}
    \item \textbf{Imagic}~\cite{Imagic} produces text embeddings that align with both the input image and the desired edit, and fine-tunes the pre-trained diffusion model to operate editing. In the implementation, we construct new text prompts to guide image editing by replacing key entities in each textual prompt, such as gender, skin color, or age. Each prompt is executed four times, ultimately yielding over 40,000 synthesized images.
    \item \textbf{Collaborative Diffusion (CoDiff)}~\cite{CoDiff} employs pre-trained uni-modal diffusion models collaborate to achieve multi-modal face generation and editing without re-training. In facial modification applications, we alter facial expressions and movements by modifying the facial segmentation masks.
    \item \textbf{Cycle Diffusion (CycleDiff)}~\cite{cyclediffusion} is a method for unpaired image-to-image translation, which presents a reconstructable encoder for stochastic diffusion probabilistic models (DPMs). We apply the modified prompts in Imagic as desired edit conditions to generate outcomes with CycleDiff.
\end{itemize}

% \footnote{\url{https://github.com/ChenWu98/cycle-diffusion}.}

\section{More Benchmarks}
\label{supsec:Benchmarks}
In this section, we first presented the specific values for \Cref{fig:subset} and \Cref{fig:linear_probing_fintune}, followed by additional experimental results. These include a further evaluation of the DiFF dataset and a new benchmark of the utilization of EGR.

\subsection{Exact Values in Figures}

\begin{table}[t]
\centering
\scalebox{0.75}{
\begin{tabular}{lcccccc}
\toprule \midrule
\multicolumn{1}{l|}{\multirow{2}{*}{Method}} & \multicolumn{1}{c|}{\multirow{2}{*}{Train}} \hspace{0.2pt} & \multicolumn{4}{c}{Testing}     \\ \cmidrule(lr){3-6} 
\multicolumn{1}{l|}{}                        & \multicolumn{1}{c|}{} \hspace{0.2pt}                       & T2I                  & \multicolumn{1}{c}{I2I} & \multicolumn{1}{c}{FS} & \multicolumn{1}{c}{FE} \\ \midrule
\multicolumn{1}{l|}{Xception}         & \multicolumn{1}{c|}{\multirow{4}{*}{T2I}} \hspace{0.2pt}  & \cellcolor[HTML]{E5E5E5}93.32 & 86.85 & 34.65 & 23.28 \\
\multicolumn{1}{l|}{F$^3$-Net}        & \multicolumn{1}{c|}{} \hspace{0.2pt}                      & \cellcolor[HTML]{E5E5E5}99.70 & 88.50 & 45.07 & 71.06 \\
\multicolumn{1}{l|}{EfficientNet}     & \multicolumn{1}{c|}{} \hspace{0.2pt}                      & \cellcolor[HTML]{E5E5E5}99.89 & 89.72 & 21.49 & 49.63  \\
\multicolumn{1}{l|}{DIRE}             & \multicolumn{1}{c|}{} \hspace{0.2pt}                      & \cellcolor[HTML]{E5E5E5}95.04 & 84.07 & 35.15 & 50.86  \\ \midrule

\multicolumn{1}{l|}{Xception}         & \multicolumn{1}{c|}{\multirow{4}{*}{I2I}} \hspace{0.2pt}  & 87.82 & \cellcolor[HTML]{E5E5E5}98.92 & 36.82 & 33.39  \\
\multicolumn{1}{l|}{F$^3$-Net}        & \multicolumn{1}{c|}{} \hspace{0.2pt}                      & 87.23 & \cellcolor[HTML]{E5E5E5}99.50 & 40.62 & 46.19  \\
\multicolumn{1}{l|}{EfficientNet}     & \multicolumn{1}{c|}{} \hspace{0.2pt}                      & 84.39 & \cellcolor[HTML]{E5E5E5}99.80 & 19.47 & 27.46  \\
\multicolumn{1}{l|}{DIRE}             & \multicolumn{1}{c|}{} \hspace{0.2pt}                      & 86.20 & \cellcolor[HTML]{E5E5E5}99.88 & 41.51 & 42.01  \\ \midrule
                                          
\multicolumn{1}{l|}{Xception}         & \multicolumn{1}{c|}{\multirow{4}{*}{FS}} \hspace{0.2pt}   & 23.17 & 24.47 & \cellcolor[HTML]{E5E5E5}99.95 & 10.17  \\
\multicolumn{1}{l|}{F$^3$-Net}        & \multicolumn{1}{c|}{} \hspace{0.2pt}                      & 35.43 & 30.39 & \cellcolor[HTML]{E5E5E5}99.98 & 20.79  \\
\multicolumn{1}{l|}{EfficientNet}     & \multicolumn{1}{c|}{} \hspace{0.2pt}                      & 16.88 & 22.17 & \cellcolor[HTML]{E5E5E5}99.87 & 10.21  \\   
\multicolumn{1}{l|}{DIRE}             & \multicolumn{1}{c|}{} \hspace{0.2pt}                      & 16.80 & 36.27 & \cellcolor[HTML]{E5E5E5}99.09 & 32.68  \\\midrule
                                          
\multicolumn{1}{l|}{Xception}         & \multicolumn{1}{c|}{\multirow{4}{*}{FE}} \hspace{0.2pt}   & 80.84 & 79.12 & 70.81 & \cellcolor[HTML]{E5E5E5} 99.95  \\
\multicolumn{1}{l|}{F$^3$-Net}        & \multicolumn{1}{c|}{} \hspace{0.2pt}                      & 82.32 & 76.92 & 56.27 & \cellcolor[HTML]{E5E5E5} 99.60  \\
\multicolumn{1}{l|}{EfficientNet}     & \multicolumn{1}{c|}{} \hspace{0.2pt}                      & 80.41 & 63.06 & 66.62 & \cellcolor[HTML]{E5E5E5} 99.24  \\
\multicolumn{1}{l|}{DIRE}             & \multicolumn{1}{c|}{} \hspace{0.2pt}                      & 56.70 & 59.22 & 43.78 & \cellcolor[HTML]{E5E5E5} 99.87  \\ \midrule \bottomrule
\end{tabular}
}
\caption{AUC (\%) comparison among re-training detectors correspond to \Cref{fig:subset}. Each row represents the performance of the model trained on a specific subset and tested on all four subsets.}
\label{Tab:Values_for_retraining}
\end{table}

\begin{table}[t]
\centering
\scalebox{0.75}{
\begin{tabular}{lcccccc}
\toprule \midrule
\multicolumn{1}{l|}{\multirow{2}{*}{Strategy}} & \multicolumn{1}{c|}{\multirow{2}{*}{Train}} \hspace{0.2pt} & \multicolumn{4}{c}{Testing}     \\ \cmidrule(lr){3-6} 
\multicolumn{1}{l|}{}                        & \multicolumn{1}{c|}{} \hspace{0.2pt}                       & T2I                  & \multicolumn{1}{c}{I2I} & \multicolumn{1}{c}{FS} & \multicolumn{1}{c}{FE} \\ \midrule
\multicolumn{1}{l|}{Re-training}         & \multicolumn{1}{c|}{\multirow{4}{*}{T2I}} \hspace{0.2pt}  & \cellcolor[HTML]{E5E5E5}93.32 & 86.85 & 34.65 & 23.28 \\
\multicolumn{1}{l|}{Linear Probing}        & \multicolumn{1}{c|}{} \hspace{0.2pt}                      & \cellcolor[HTML]{E5E5E5}71.36 & 74.75 & 65.83 & 66.41 \\
\multicolumn{1}{l|}{Fine-Tuning}     & \multicolumn{1}{c|}{} \hspace{0.2pt}                      & \cellcolor[HTML]{E5E5E5}93.66 & 88.94 & 36.10 & 37.51  \\ \midrule

\multicolumn{1}{l|}{Re-training}         & \multicolumn{1}{c|}{\multirow{4}{*}{I2I}} \hspace{0.2pt}  & 87.82 & \cellcolor[HTML]{E5E5E5}98.92 & 36.82 & 33.39  \\
\multicolumn{1}{l|}{Linear Probing}        & \multicolumn{1}{c|}{} \hspace{0.2pt}                      & 79.88 & \cellcolor[HTML]{E5E5E5}85.88 & 87.68 & 76.23  \\
\multicolumn{1}{l|}{Fine-Tuning}     & \multicolumn{1}{c|}{} \hspace{0.2pt}                      & 97.79 & \cellcolor[HTML]{E5E5E5}98.76 & 61.64 & 48.33  \\ \midrule
                                          
\multicolumn{1}{l|}{Re-training}         & \multicolumn{1}{c|}{\multirow{4}{*}{FS}} \hspace{0.2pt}   & 23.17 & 24.47 & \cellcolor[HTML]{E5E5E5}99.95 & 10.17  \\
\multicolumn{1}{l|}{Linear Probing}        & \multicolumn{1}{c|}{} \hspace{0.2pt}                    & 60.77 & 66.45 & \cellcolor[HTML]{E5E5E5}92.93 & 60.78  \\
\multicolumn{1}{l|}{Fine-Tuning}     & \multicolumn{1}{c|}{} \hspace{0.2pt}                          & 18.04 & 24.71 & \cellcolor[HTML]{E5E5E5}99.44 & 16.48  \\ \midrule
                                    
\multicolumn{1}{l|}{Re-training}         & \multicolumn{1}{c|}{\multirow{4}{*}{FE}} \hspace{0.2pt}   & 80.84 & 79.12 & 70.81 & \cellcolor[HTML]{E5E5E5} 99.95  \\
\multicolumn{1}{l|}{Linear Probing}        & \multicolumn{1}{c|}{} \hspace{0.2pt}                      & 56.52 & 65.54 & 82.52 & \cellcolor[HTML]{E5E5E5} 78.13  \\
\multicolumn{1}{l|}{Fine-Tuning}     & \multicolumn{1}{c|}{} \hspace{0.2pt}                      & 89.74 & 74.10 & 75.96 & \cellcolor[HTML]{E5E5E5} 99.93  \\ \midrule \bottomrule
\end{tabular}
}
\caption{AUC (\%) of Xception with different training strategies correspond to \Cref{fig:linear_probing_fintune}. Each row represents the performance of the model trained on a specific subset and tested on all four subsets.}
\label{Tab:Values_for_retraining_lb_ft}
\end{table}

\Cref{Tab:Values_for_retraining} and \Cref{Tab:Values_for_retraining_lb_ft} correspond to the specific values of \Cref{fig:subset} and \Cref{fig:linear_probing_fintune}, respectively.

\subsection{Results on Full DiFF}

\begin{table}[t]
\centering
\scalebox{0.75}{
\begin{tabular}{lccccccc}
\toprule \midrule
\multicolumn{2}{l|}{Method} & \multicolumn{1}{c|}{Train} \hspace{0.2pt} & \multicolumn{2}{c}{Tesing Subset}     \\ \cmidrule(lr){1-2}  \cmidrule(lr){4-5} 
\multicolumn{1}{l|}{Backone}  & \multicolumn{1}{c|}{+EGR}    & \multicolumn{1}{c|}{Subset} \hspace{0.2pt}  & Full & Others \\ \midrule
\multicolumn{1}{l|}{Xception}       &\multicolumn{1}{c|}{$\times$}  & \multicolumn{1}{c|}{\multirow{8}{*}{T2I}} \hspace{0.2pt}  & 71.23    & 50.18   \\
\multicolumn{1}{l|}{Xception}       &\multicolumn{1}{c|}{\checkmark}  & \multicolumn{1}{c|}{}  \hspace{0.2pt}                     & \textbf{81.07}    & \textbf{68.17}   \\
\multicolumn{1}{l|}{F$^3$-Net}      &\multicolumn{1}{c|}{$\times$}  & \multicolumn{1}{c|}{} \hspace{0.2pt}                      & 72.41    & 58.56  \\
\multicolumn{1}{l|}{F$^3$-Net}      &\multicolumn{1}{c|}{\checkmark}  & \multicolumn{1}{c|}{} \hspace{0.2pt}                      & \textbf{80.97}    & \textbf{66.50 }  \\
\multicolumn{1}{l|}{EfficientNet}   &\multicolumn{1}{c|}{$\times$} & \multicolumn{1}{c|}{}  \hspace{0.2pt}                      & 79.36    & 60.02 \\
\multicolumn{1}{l|}{EfficientNet}   &\multicolumn{1}{c|}{\checkmark}  & \multicolumn{1}{c|}{}  \hspace{0.2pt}                      & \textbf{80.37}    & \textbf{62.87} \\
\multicolumn{1}{l|}{DIRE}           &\multicolumn{1}{c|}{$\times$} & \multicolumn{1}{c|}{}  \hspace{0.2pt}                      & 66.85    & 53.28 \\
\multicolumn{1}{l|}{DIRE}   &\multicolumn{1}{c|}{\checkmark} & \multicolumn{1}{c|}{}  \hspace{0.2pt}                              & \textbf{72.38}    & \textbf{54.37}\\\midrule

\multicolumn{1}{l|}{Xception}       &\multicolumn{1}{c|}{$\times$}  & \multicolumn{1}{c|}{\multirow{8}{*}{I2I}} \hspace{0.2pt}  & 78.01    & 73.78   \\
\multicolumn{1}{l|}{Xception}       &\multicolumn{1}{c|}{\checkmark}  & \multicolumn{1}{c|}{} \hspace{0.2pt}                       & \textbf{84.26}    & \textbf{81.10}   \\
\multicolumn{1}{l|}{F$^3$-Net}      &\multicolumn{1}{c|}{$\times$}  & \multicolumn{1}{c|}{} \hspace{0.2pt}                       & 78.76    & 72.78   \\
\multicolumn{1}{l|}{F$^3$-Net}      &\multicolumn{1}{c|}{\checkmark}  & \multicolumn{1}{c|}{} \hspace{0.2pt}                       & \textbf{79.28}    & \textbf{76.22}   \\
\multicolumn{1}{l|}{EfficientNet}   &\multicolumn{1}{c|}{$\times$} & \multicolumn{1}{c|}{}  \hspace{0.2pt}                       & 75.61   & 70.73 \\
\multicolumn{1}{l|}{EfficientNet}   &\multicolumn{1}{c|}{\checkmark} & \multicolumn{1}{c|}{}  \hspace{0.2pt}                       & \textbf{88.85}    & \textbf{86.75} \\
\multicolumn{1}{l|}{DIRE}           &\multicolumn{1}{c|}{$\times$} & \multicolumn{1}{c|}{}  \hspace{0.2pt}                       & 76.54    &73.57  \\
\multicolumn{1}{l|}{DIRE}   &\multicolumn{1}{c|}{\checkmark} & \multicolumn{1}{c|}{}  \hspace{0.2pt}                               & \textbf{84.94} &\textbf{82.16} \\\midrule
                                          
\multicolumn{1}{l|}{Xception}       &\multicolumn{1}{c|}{$\times$}  & \multicolumn{1}{c|}{\multirow{8}{*}{FS}} \hspace{0.2pt}  & 37.47    & 22.58   \\
\multicolumn{1}{l|}{Xception}       &\multicolumn{1}{c|}{\checkmark}  & \multicolumn{1}{c|}{} \hspace{0.2pt}                      & \textbf{68.45}   & \textbf{60.93}  \\
\multicolumn{1}{l|}{F$^3$-Net}      &\multicolumn{1}{c|}{$\times$}  & \multicolumn{1}{c|}{} \hspace{0.2pt}                      & 46.36   & 33.62   \\
\multicolumn{1}{l|}{F$^3$-Net}      &\multicolumn{1}{c|}{\checkmark}  & \multicolumn{1}{c|}{} \hspace{0.2pt}                      & \textbf{77.51}   & \textbf{66.32}   \\
\multicolumn{1}{l|}{EfficientNet}   &\multicolumn{1}{c|}{$\times$} & \multicolumn{1}{c|}{}  \hspace{0.2pt}                       & 34.73   & 17.38  \\
\multicolumn{1}{l|}{EfficientNet}   &\multicolumn{1}{c|}{\checkmark} & \multicolumn{1}{c|}{}  \hspace{0.2pt}                       & \textbf{65.19}   & \textbf{56.89} \\
\multicolumn{1}{l|}{DIRE}           &\multicolumn{1}{c|}{$\times$} & \multicolumn{1}{c|}{}  \hspace{0.2pt}                       & 69.23 & 58.35 \\
\multicolumn{1}{l|}{DIRE}   &\multicolumn{1}{c|}{\checkmark} & \multicolumn{1}{c|}{}  \hspace{0.2pt}                               & \textbf{74.67}    & \textbf{69.62} \\\midrule
                                          
\multicolumn{1}{l|}{Xception}       &\multicolumn{1}{c|}{$\times$}  & \multicolumn{1}{c|}{\multirow{8}{*}{FE}} \hspace{0.2pt}  & 87.97    & 85.78   \\
\multicolumn{1}{l|}{Xception}       &\multicolumn{1}{c|}{\checkmark}  & \multicolumn{1}{c|}{} \hspace{0.2pt}                     & \textbf{89.30}    & \textbf{87.35}   \\
\multicolumn{1}{l|}{F$^3$-Net}      &\multicolumn{1}{c|}{$\times$}  & \multicolumn{1}{c|}{} \hspace{0.2pt}                      & 81.69   & 80.70   \\
\multicolumn{1}{l|}{F$^3$-Net}      &\multicolumn{1}{c|}{\checkmark}  & \multicolumn{1}{c|}{} \hspace{0.2pt}                      & \textbf{87.21}   & \textbf{84.91}  \\
\multicolumn{1}{l|}{EfficientNet}   &\multicolumn{1}{c|}{$\times$} & \multicolumn{1}{c|}{}  \hspace{0.2pt}                      & 81.96   & 78.67 \\
\multicolumn{1}{l|}{EfficientNet}   &\multicolumn{1}{c|}{\checkmark} & \multicolumn{1}{c|}{}  \hspace{0.2pt}                      & \textbf{83.62}   & \textbf{80.63}  \\
\multicolumn{1}{l|}{DIRE}   &\multicolumn{1}{c|}{$\times$} & \multicolumn{1}{c|}{}  \hspace{0.2pt}                              & {81.06}   & {78.35} \\
\multicolumn{1}{l|}{DIRE}   &\multicolumn{1}{c|}{\checkmark} & \multicolumn{1}{c|}{}  \hspace{0.2pt}                              & \textbf{88.79}   & \textbf{83.26} \\ \midrule \bottomrule
\end{tabular}
}
\caption{AUC (\%) comparison among re-trained detectors when tested full DiFF (\ie, four subsets) or full DiFF without training subset (\ie, three subsets).}
\label{Tab:Full_DiFF}
\end{table}

\begin{table}[t]
\centering
\scalebox{0.75}{
\begin{tabular}{lccccccc}
\toprule \midrule
\multicolumn{1}{l|}{\multirow{2}{*}{Method}} & \multicolumn{1}{c|}{\multirow{2}{*}{Train}} \hspace{0.2pt} & \multicolumn{2}{c}{Training Strategy}     \\ \cmidrule(lr){3-4} 
\multicolumn{1}{l|}{}    & \multicolumn{1}{c|}{Dataset} \hspace{0.2pt}  & Baseline & \multicolumn{1}{c}{EGR}  \\ \midrule
\multicolumn{1}{l|}{Xception}         & \multicolumn{1}{c|}{\multirow{4}{*}{DiFF}} \hspace{0.2pt} & 93.87    & \textbf{97.81}  \\
\multicolumn{1}{l|}{F$^3$-Net}        & \multicolumn{1}{c|}{} \hspace{0.2pt}                      & 98.37    & \textbf{99.05}  \\
\multicolumn{1}{l|}{EfficientNet}     & \multicolumn{1}{c|}{} \hspace{0.2pt}                      & 94.34    & \textbf{99.26} \\
\multicolumn{1}{l|}{DIRE}             & \multicolumn{1}{c|}{} \hspace{0.2pt}                      & 96.35    & \textbf{98.62} \\ 
\midrule \bottomrule
\end{tabular}
}
\caption{AUC (\%) comparison among re-trained detectors. Each row represents the performance when trained and tested on full DiFF dataset.}
\label{Tab:trained_Full_Diff}
\end{table}

\noindent\textbf{Trained on single subset.}
In \Cref{Tab:Full_DiFF}, we presented the test results on the complete DiFF dataset (\ie, across all subsets) following training on a single subset. Furthermore, we reported on the performance of the model when trained on one subset and tested on a combination of other subsets (\eg, trained on T2I and tested on I2I+FS+FE).
It can be observed that the EGR method significantly increases the detection performance of the models, which is consistent with the observations from \Cref{Tab:subset_with_EGR}.

\noindent\textbf{Trained on full DiFF.}
We also evaluated the models' performance when trained and tested on the complete DiFF dataset, with the experimental results depicted in \Cref{Tab:trained_Full_Diff}.
We observed that when the distributions of the training and test sets are identical, the models are capable of achieving satisfactory performance, and the implementation of EGR can enhance the model to a certain extent. However, it is noteworthy that this evaluation strategy does not reflect the detectors' generalizability. In fact, drawing from previous experimental results (\eg, \Cref{Tab:subset_with_EGR} and \Cref{Tab:Full_DiFF}), we are aware that the generalizability of the current detectors presents a significant challenge. This issue lies at the heart of the current issues on the detection of forged images. Therefore, we advocate for the validation of detectors based on their performance when trained on a single subset and subsequently tested on multiple unseen subsets.

\subsection{Detection with Post-processing Methods}

% \begin{figure}
%     \centering
%     \includegraphics[width=0.45\textwidth]{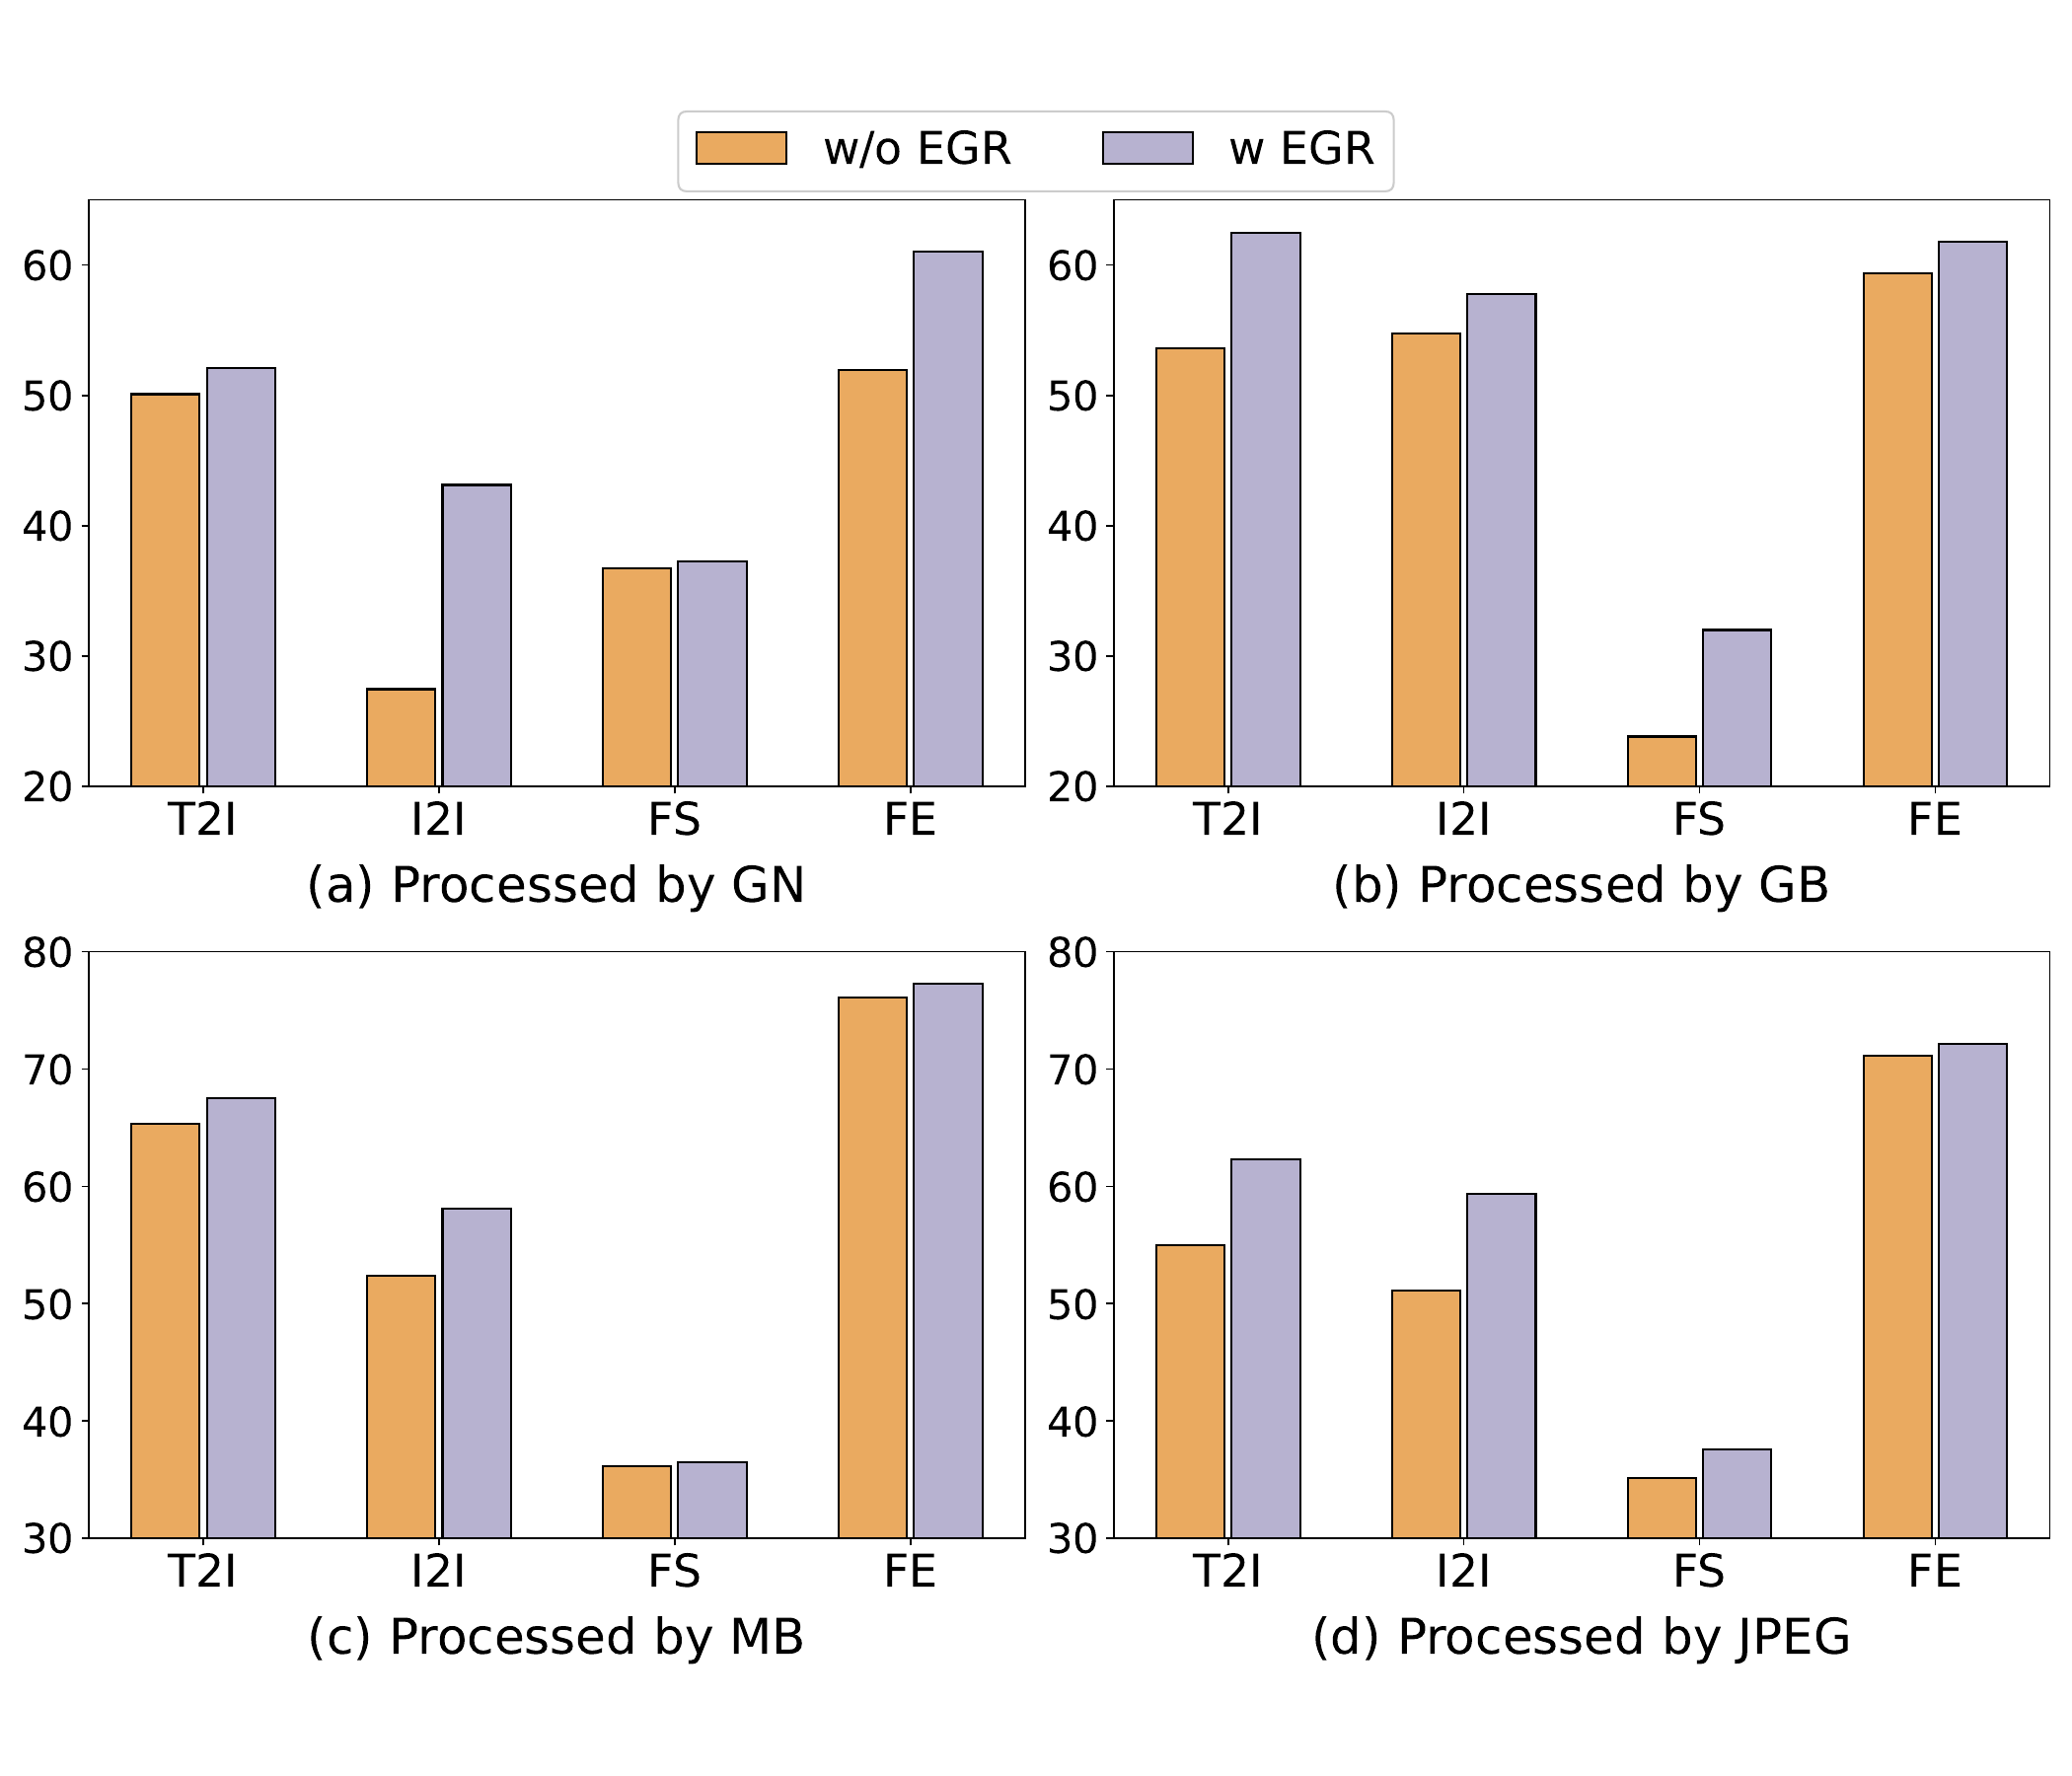}
%     \caption{Avarage AUCs (\%) of EfficientNet subjected to several post-processing methods. X-axis: training subset.}
%     \label{fig:post-processing}
% \end{figure}

\begin{table}[t]
\centering
\scalebox{0.72}{
\begin{tabular}{lc|ccccccc}
\toprule \midrule
\multicolumn{1}{l|}{\multirow{2}{*}{Method}} & \multicolumn{1}{l|}{\multirow{2}{*}{+EGR}} & \multicolumn{1}{c|}{\multirow{2}{*}{Train}} \hspace{0.2pt} & \multicolumn{4}{c}{Processing Method}     \\ \cmidrule(lr){4-7} 
\multicolumn{1}{l|}{}  & \multicolumn{1}{l|}{}  & \multicolumn{1}{c|}{Subset} \hspace{0.2pt}  & \multicolumn{1}{c}{GN} & \multicolumn{1}{c}{GB} & \multicolumn{1}{c}{MB} & \multicolumn{1}{c}{JPEG}\\ \midrule
\multicolumn{1}{l|}{Xception}     & $\times$   & \multicolumn{1}{c|}{\multirow{4}{*}{T2I}} \hspace{0.2pt}      & 47.65 & 15.02 & 56.59 & 58.69  \\
\multicolumn{1}{l|}{Xception}     & \checkmark  & \multicolumn{1}{c|}{} \hspace{0.2pt}                         & \textbf{62.49} & \textbf{32.38} & \textbf{70.87} & \textbf{70.69}  \\
\multicolumn{1}{l|}{EfficientNet} & $\times$   & \multicolumn{1}{c|}{} \hspace{0.2pt}                          & 40.09 & 53.62 & 65.35 & 54.98\\
\multicolumn{1}{l|}{EfficientNet} & \checkmark  & \multicolumn{1}{c|}{} \hspace{0.2pt}                         & \textbf{42.10} & \textbf{62.47} & \textbf{69.51} & \textbf{62.28}\\ \midrule

\multicolumn{1}{l|}{Xception}     & $\times$   & \multicolumn{1}{c|}{\multirow{4}{*}{I2I}} \hspace{0.2pt}     & 19.70 & 54.09 & 58.07 & 63.66\\
\multicolumn{1}{l|}{Xception}    & \checkmark   & \multicolumn{1}{c|}{} \hspace{0.2pt}                       & \textbf{63.19} & \textbf{54.84} & \textbf{70.13} & \textbf{70.25} \\
\multicolumn{1}{l|}{EfficientNet} & $\times$   & \multicolumn{1}{c|}{} \hspace{0.2pt}                          & 27.76 & 54.75 & 52.39 & 51.01\\
\multicolumn{1}{l|}{EfficientNet}         & \checkmark   & \multicolumn{1}{c|}{} \hspace{0.2pt}                 & \textbf{43.13} & \textbf{77.32} & \textbf{68.13} & \textbf{59.39}\\ \midrule
                                          
\multicolumn{1}{l|}{Xception}     & $\times$   & \multicolumn{1}{c|}{\multirow{4}{*}{FS}} \hspace{0.2pt}       & 35.40 & 34.82 & 38.58 & 37.73\\
\multicolumn{1}{l|}{Xception}    & \checkmark   & \multicolumn{1}{c|}{} \hspace{0.2pt}                        & \textbf{58.59} & \textbf{48.49} & \textbf{58.30} & \textbf{66.36} \\
\multicolumn{1}{l|}{EfficientNet} & $\times$   & \multicolumn{1}{c|}{} \hspace{0.2pt}                          & 36.74 & 23.82 & 36.12 & 35.13\\   
\multicolumn{1}{l|}{EfficientNet}         & \checkmark   & \multicolumn{1}{c|}{} \hspace{0.2pt}                 & \textbf{49.27} & \textbf{32.01} & \textbf{36.51} & \textbf{45.57}\\\midrule
                                          
\multicolumn{1}{l|}{Xception}     & $\times$   & \multicolumn{1}{c|}{\multirow{4}{*}{FE}} \hspace{0.2pt}      & 39.69 & 24.15 & 79.35 & 81.19 \\
\multicolumn{1}{l|}{Xception}    & \checkmark   & \multicolumn{1}{c|}{} \hspace{0.2pt}                        & \textbf{57.99} & \textbf{25.51} & \textbf{87.71} & \textbf{87.52} \\
\multicolumn{1}{l|}{EfficientNet} & $\times$   & \multicolumn{1}{c|}{} \hspace{0.2pt}                         & 51.95 & 39.65 & 71.10 & 71.14 \\
\multicolumn{1}{l|}{EfficientNet}         & \checkmark   & \multicolumn{1}{c|}{} \hspace{0.2pt}               & \textbf{61.04} & \textbf{39.74} & \textbf{74.30} & \textbf{72.11}\\ \midrule \bottomrule
\end{tabular}
}
\caption{AUC (\%) comparison of detectors with and without our EGR method with different post-processing methods. Each row represents the average performance when tested on all four DiFF subsets. Better results are highlighted in bold.
\emph{GN}: Gaussian Noise;
\emph{GB}: Gaussian Blur;
\emph{MB}: Median Blur;
\emph{JPEG}: JPEG Compression.}
\label{Tab:EGR_post_process}
\end{table}

\noindent\textbf{Results of EGR with post-processing approaches.}
We also evaluated the performance of models incorporating EGR when dealing with several post-processing approaches. As demonstrated in \Cref{Tab:EGR_post_process}, EGR enhances the models' robustness for four different post-processing approaches. For instance, when the EfficientNet is trained on I2I, integrating EGR results in an average AUC improvement of 10\%. This can be attributed to EGR guiding the models' attention to high-level features such as facial contours. These features offer more reliable evidence for distinguishing genuine from forged faces after post-processing.

\subsection{More Ablation Study on EGR}

\begin{figure}[t]
    \centering
    \includegraphics[width=0.45\textwidth]{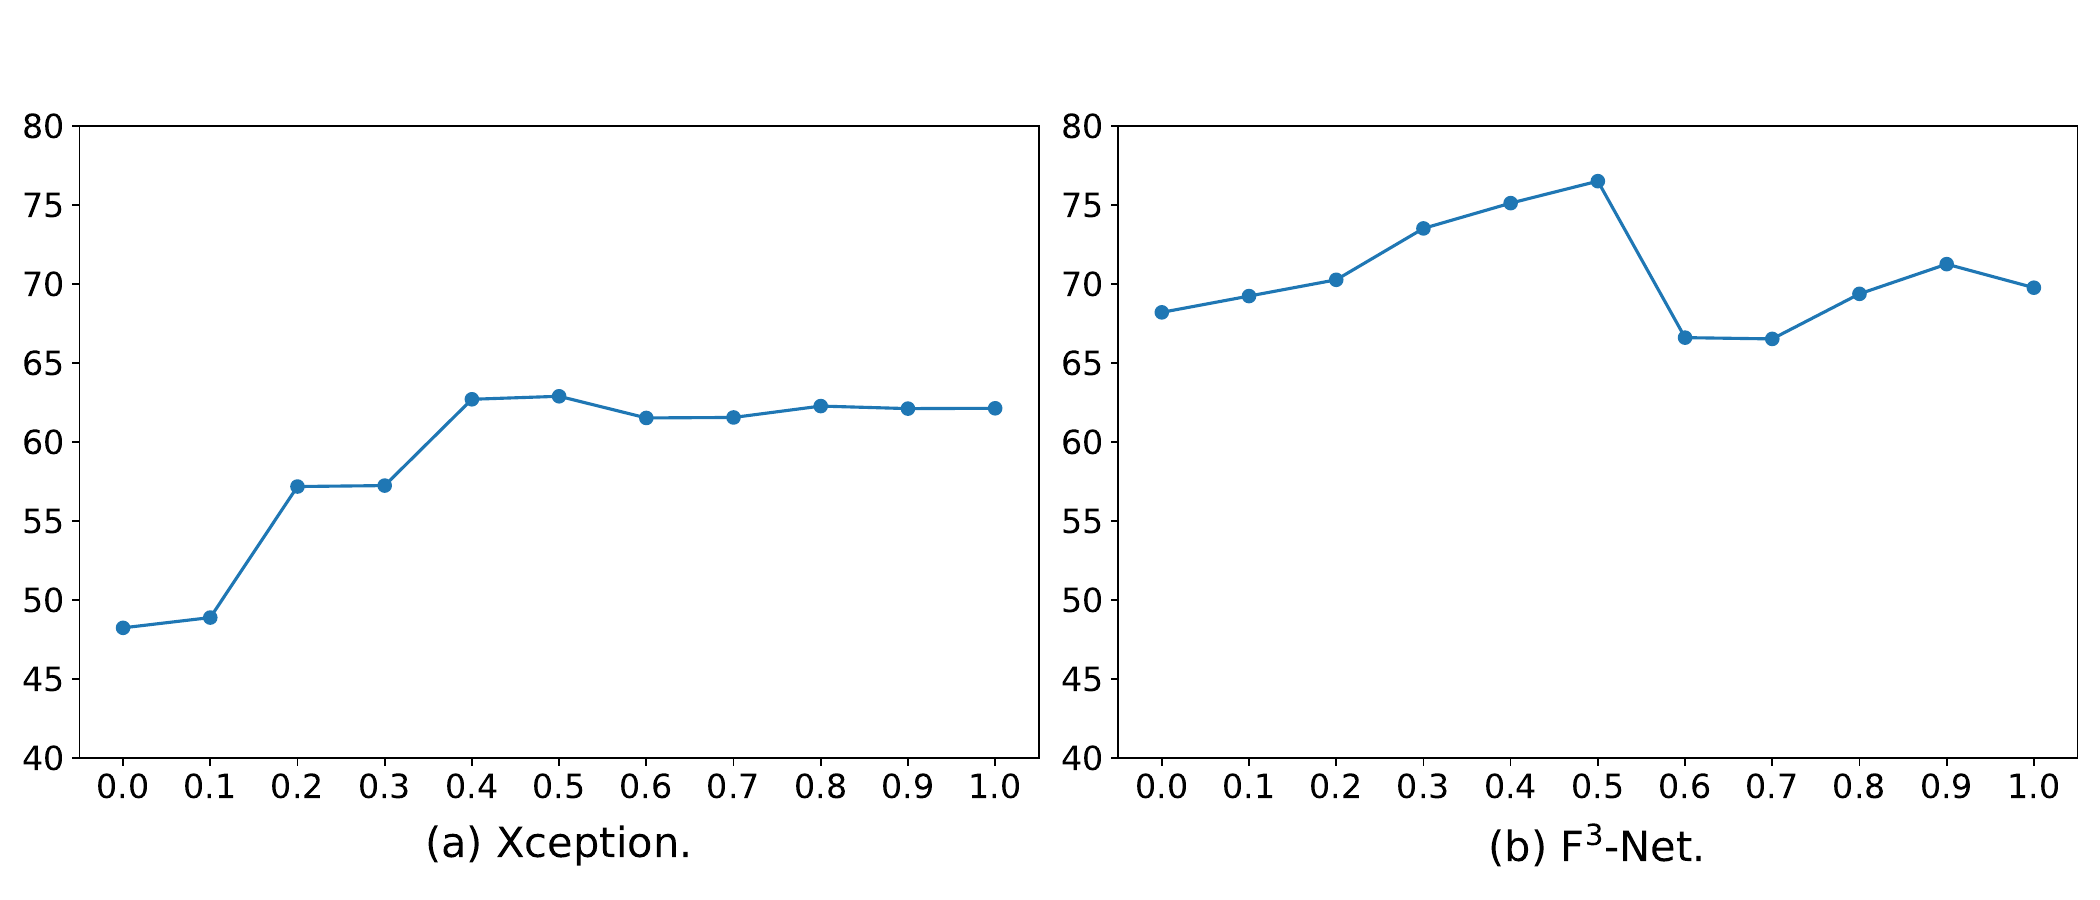}
    \caption{AUCs (\%) of (a) Xception and (b) F$^3$-Net. All of the models are trained on the T2I subset and tested on the other three subsets. Y-axis: Average AUC of detectors aross three subsets.}
    \label{fig:lambda_test}
\end{figure}

\noindent\textbf{Studies on parameter $\lambda$ of EGR.} 
We evaluated the impact of varying values of $\lambda$ in \Cref{Eqn: regular}. 
Specifically, we utilized T2I as the training subset and assessed the average AUC across the remaining three subsets.
\Cref{fig:lambda_test} shows that as the value of $\lambda$ increases, the models' performance gradually improves and stabilizes when $\lambda$ reaches 0.5. Beyond this value, there's a minor decline in AUC. there is a slight decrease in AUC. This may be attributed to the model excessively emphasizing edge graphs, potentially overlooking the color and texture features in pristine images.

\begin{figure}[t]
    \centering
    \includegraphics[width=0.42\textwidth]{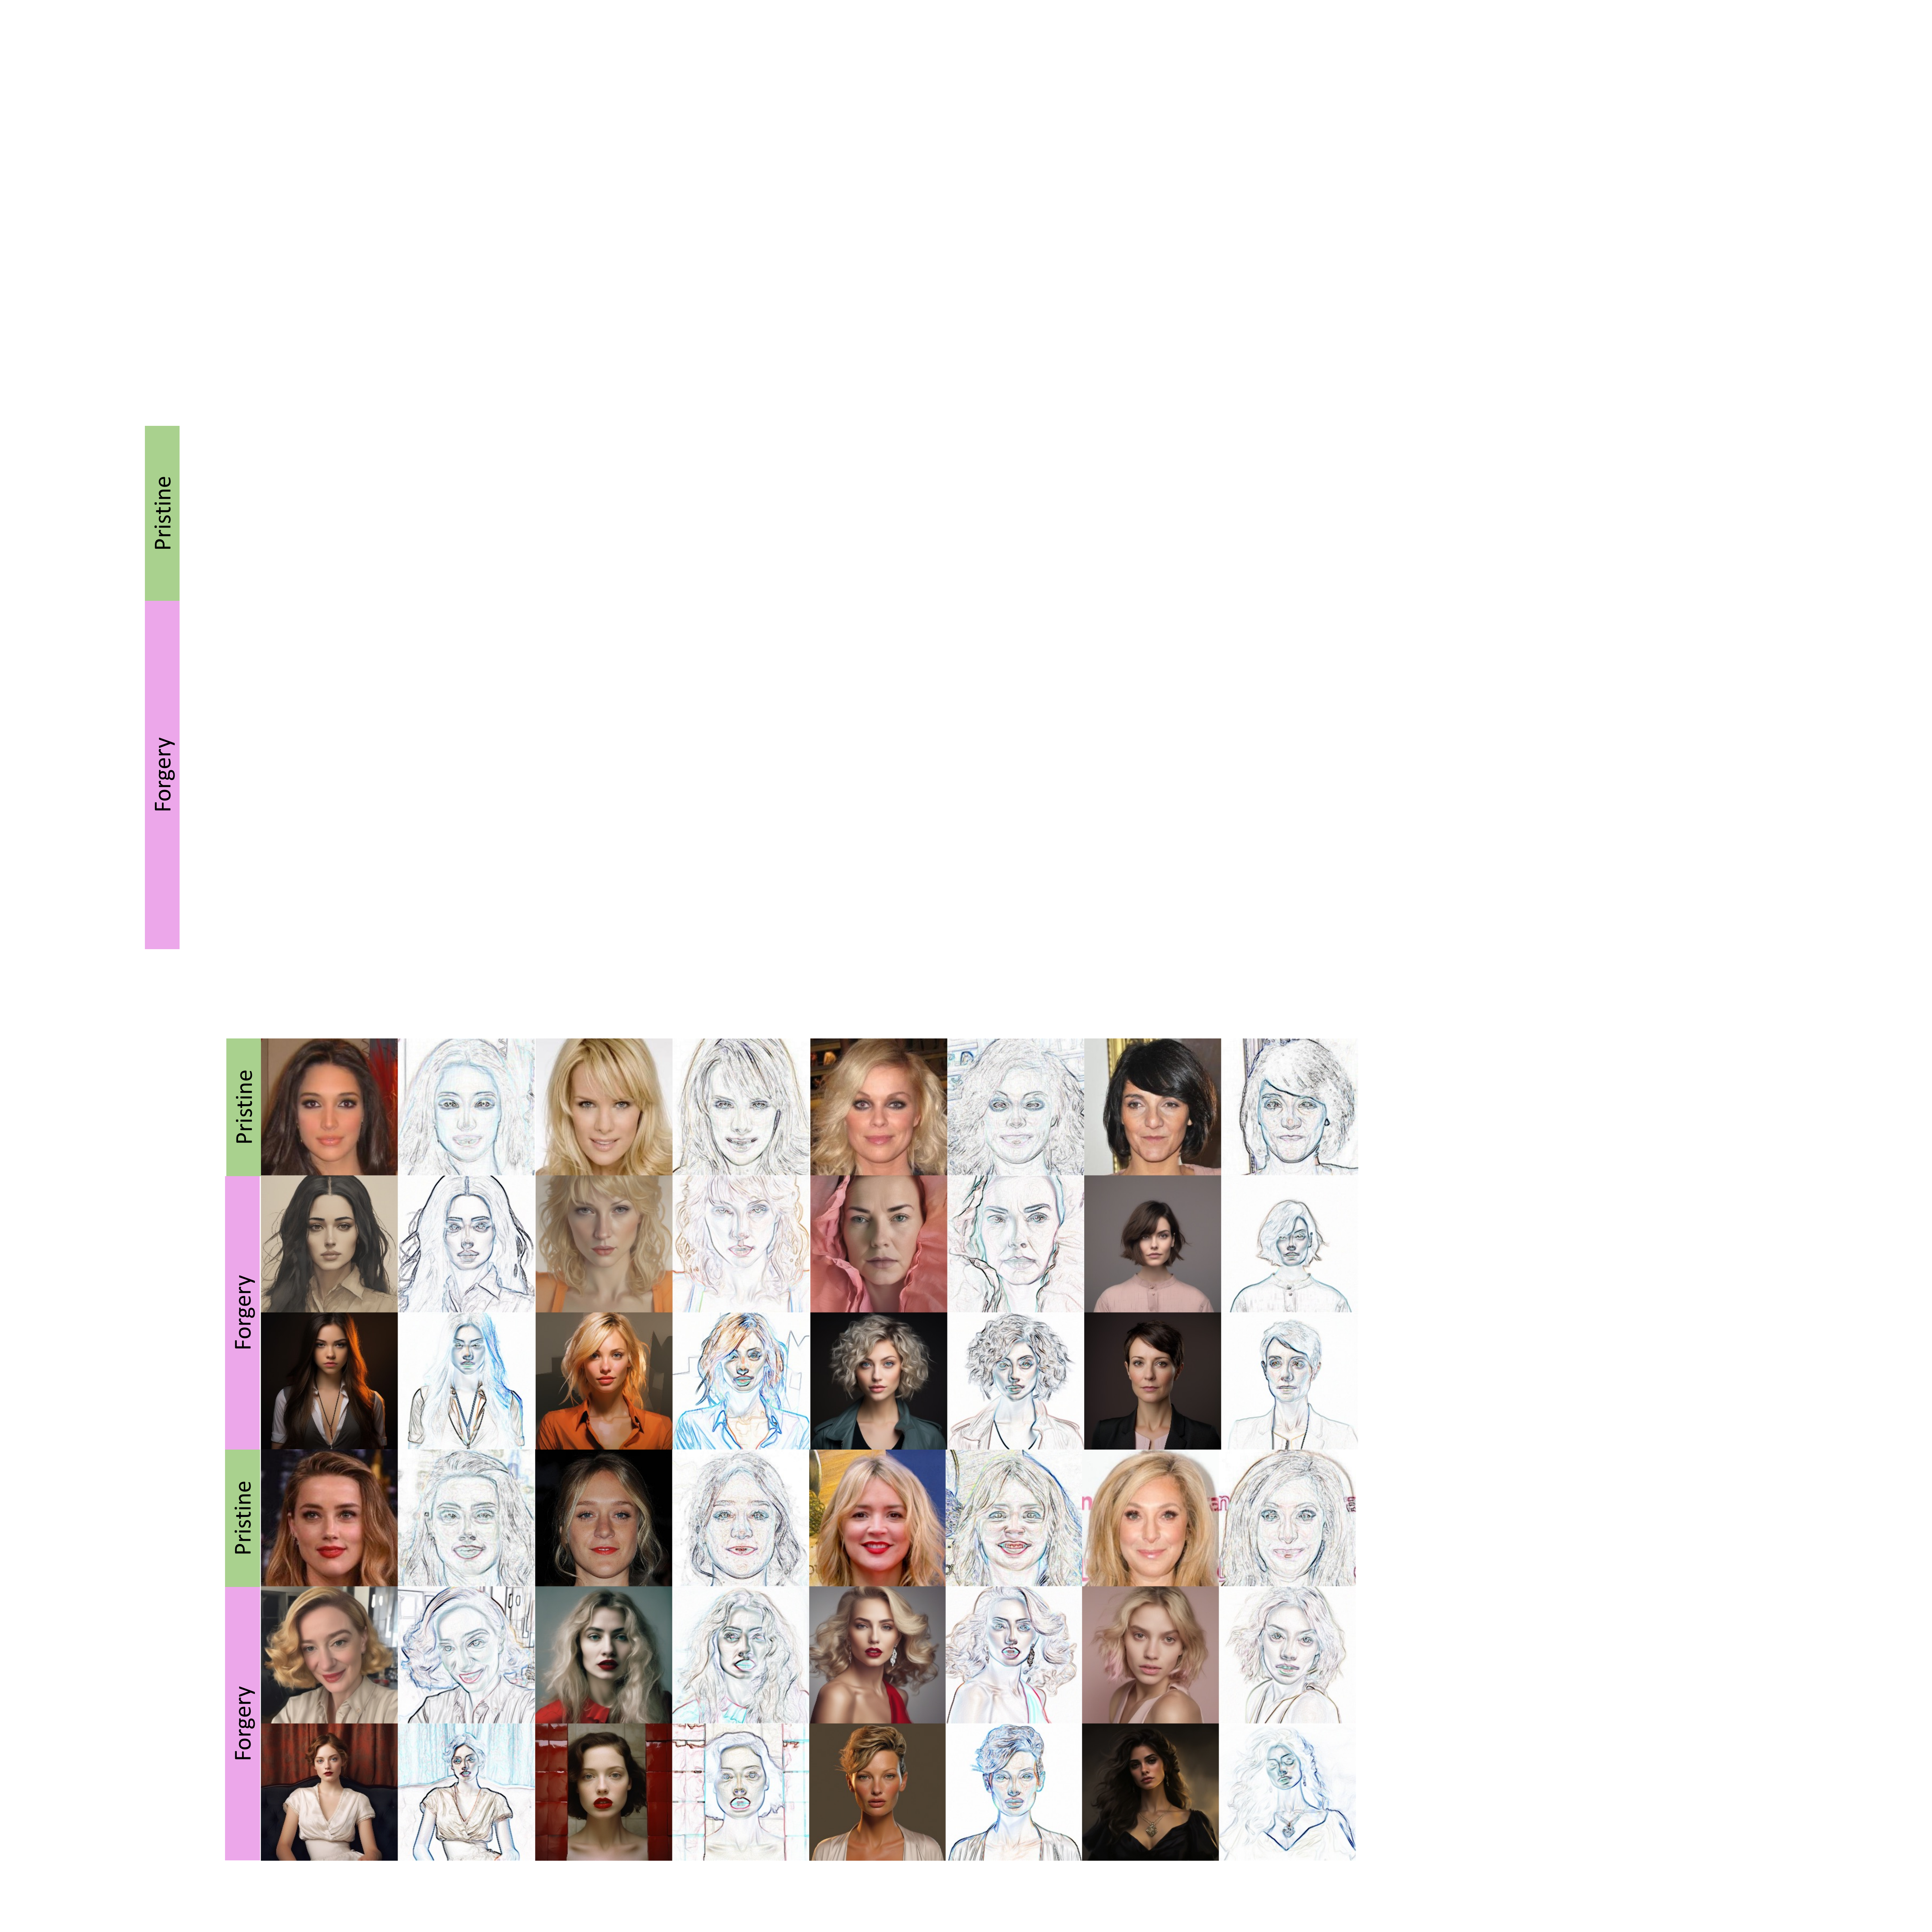}
    \caption{More edge graphs from DiFF.}
    \label{fig:edges}
\end{figure}

\begin{figure*}[t]
    \centering
    \includegraphics[width=0.95\textwidth]{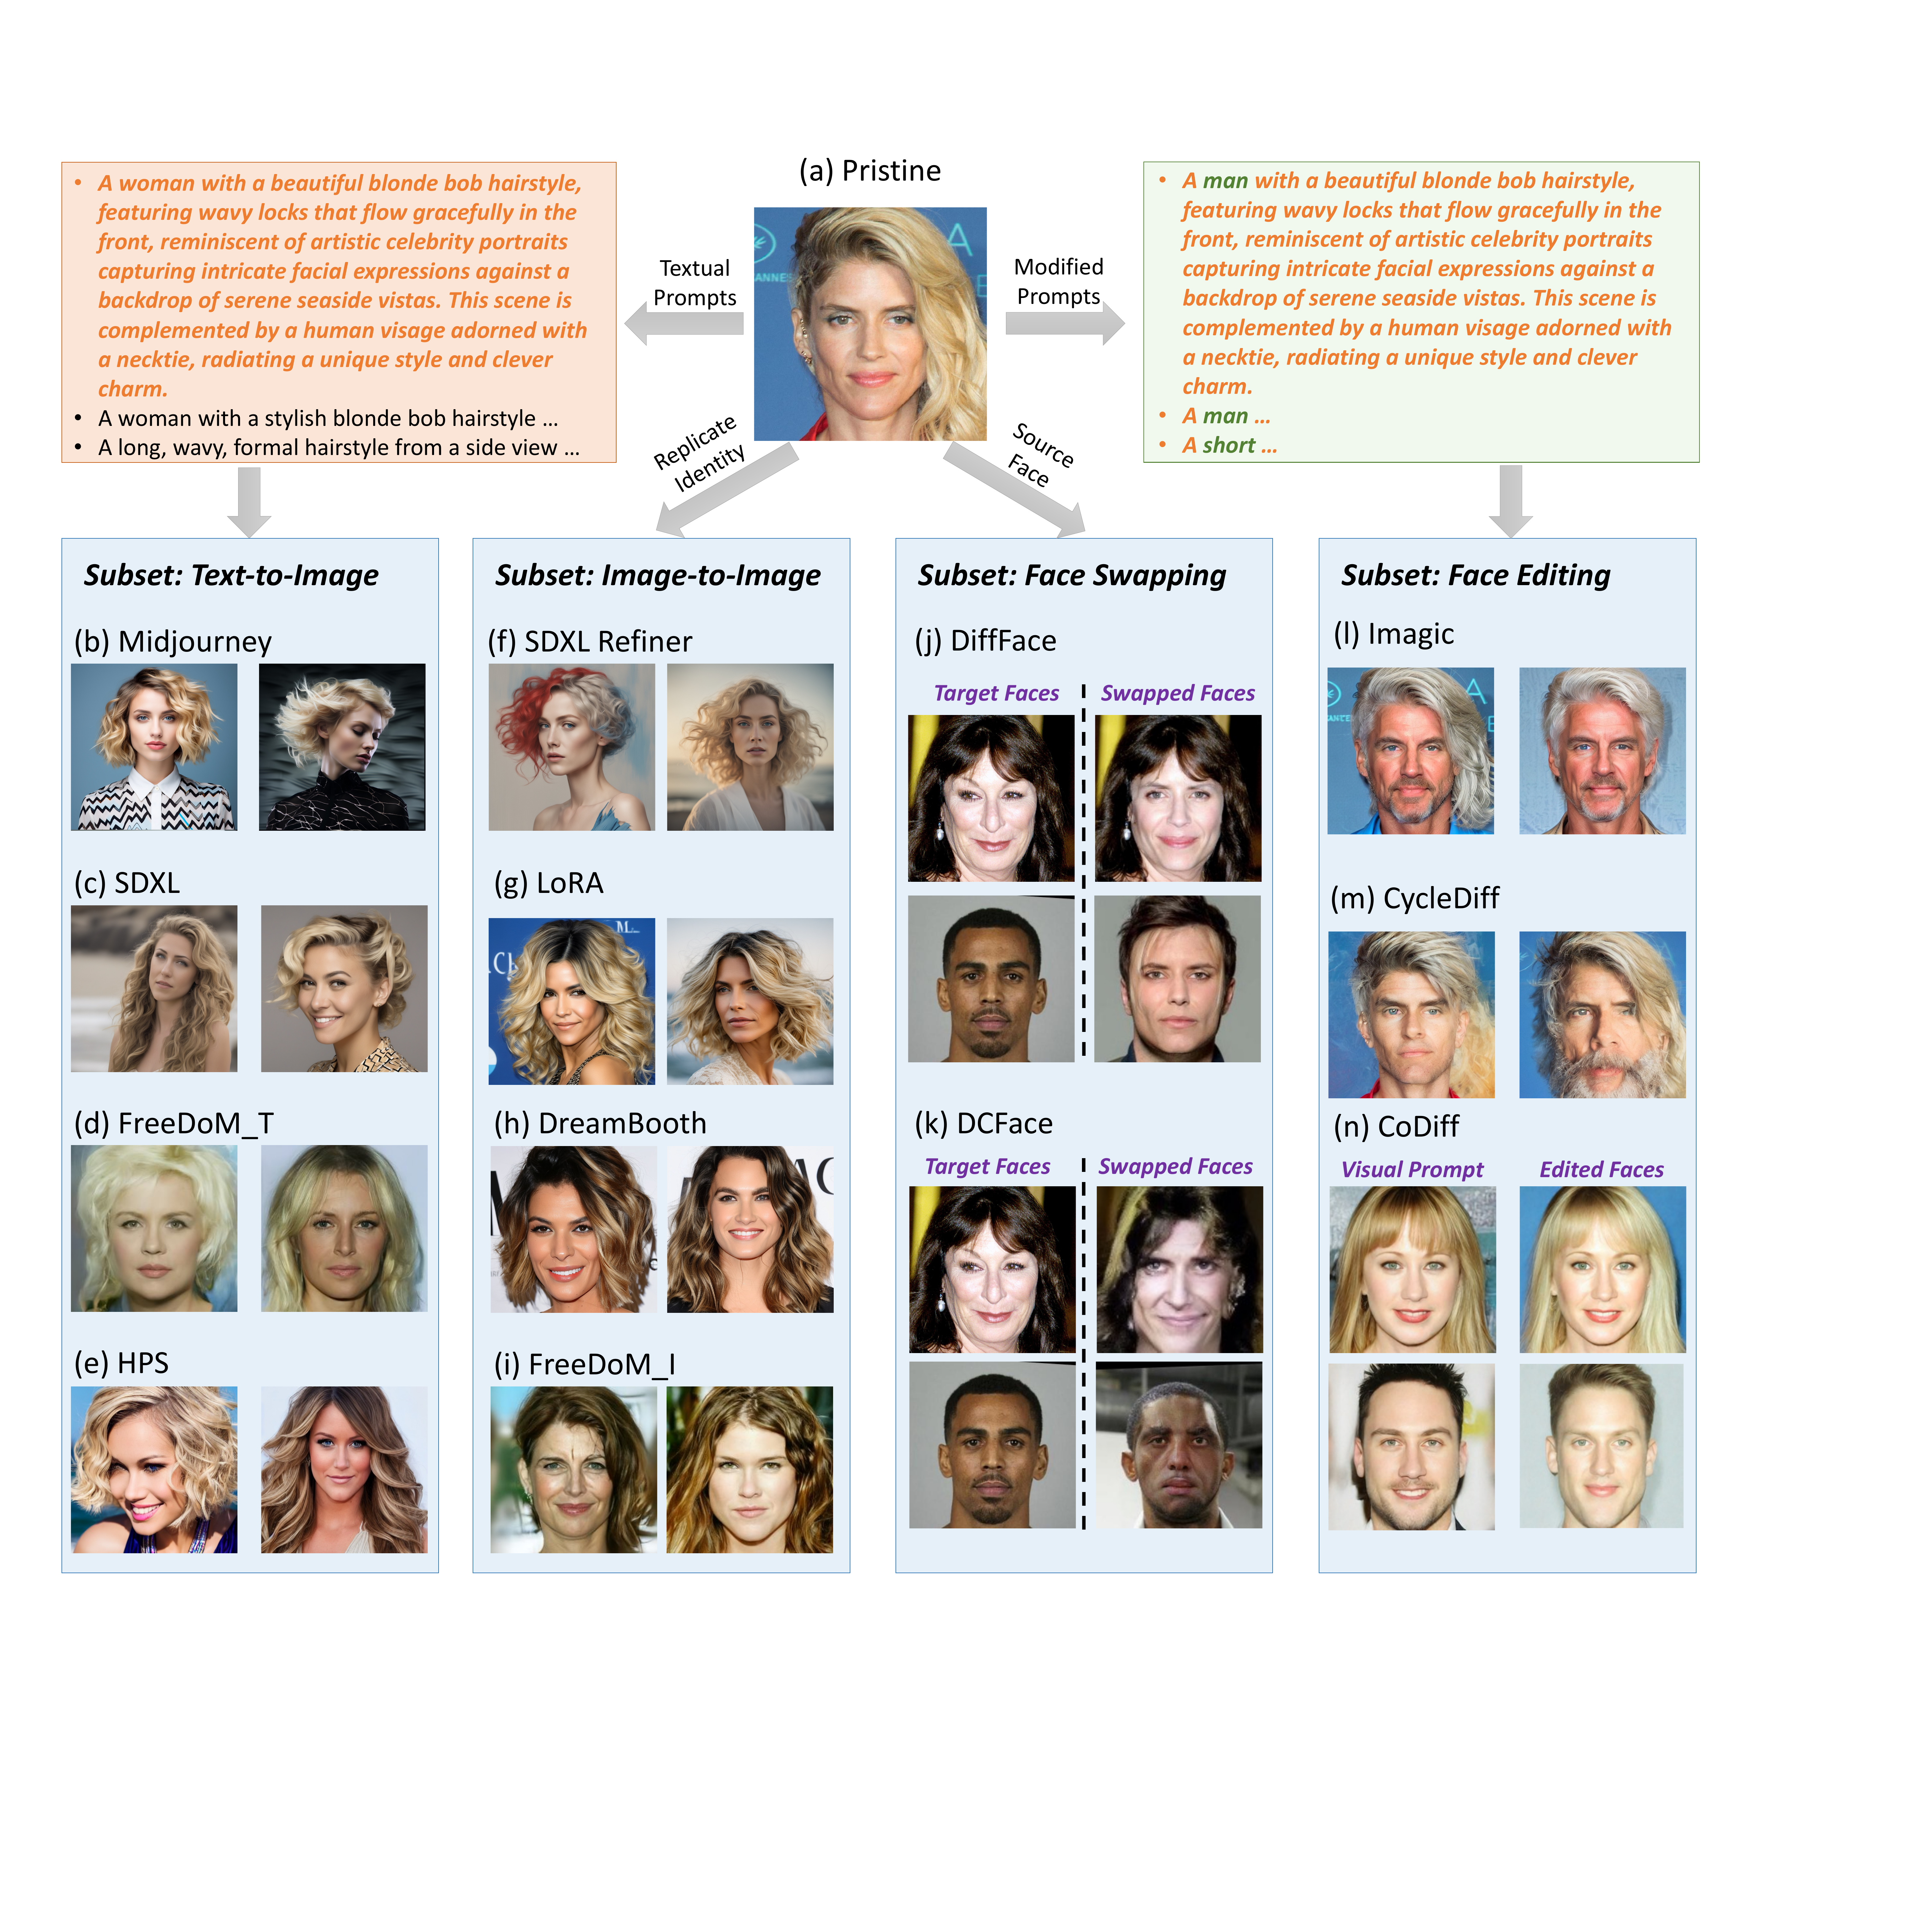}
    \caption{Visualization of one sample from DiFF. All synthesized images can be associated with the pristine images through textual or visual prompts.}
    \label{fig:Visual_Full}
\end{figure*}

\section{Visualizations of DiFF}
\label{supsec:Visualizations}

\subsection{Edge Graphs}

In \Cref{fig:edges}, we present more edge graphs. Furthermore, we offer a detailed explanation of the extraction for edge graphs. Specifically, we employ the Sobel operator to capture the edge graphs~\cite{edge_graphs}.
The Sobel operator is an influential technique in image processing. This operator functions by accentuating regions of high frequency, which correspond to edges. The core of the Sobel operator lies in its use of two distinct 3x3 kernels, each designed for detecting horizontal and vertical edges.

For horizontal edge detection:
\begin{equation}
M_x=\left(\begin{array}{lll}
-1 & 0 & 1 \\
-2 & 0 & 2 \\
-1 & 0 & 1
\end{array}\right).
\end{equation}

For vertical edge detection:
\begin{equation}
M_y=\left(\begin{array}{lll}
-1 & -2 & -1 \\
0 & 0 & 0 \\
1 & 2 & 1
\end{array}\right).
\end{equation}

Each pixel in the image is subjected to both kernels by superimposing them on the pixel and its immediate neighbors. This operation essentially computes a weighted average, accentuating changes in intensity across the specified directions. The gradient magnitude at each pixel is ascertained by integrating the results from both horizontal and vertical convolutions. This is typically computed using the formula:
\begin{equation}
G=\sqrt{G_x^2+G_y^2},
\end{equation}
where $G_x$ and $G_y$ represents the result of the horizontal and vertical convolution, respectively.
Furthermore, the direction of the gradient can be calculated at each pixel, which offers insights into the orientation of edges. By establishing a threshold, gradients exceeding this value are classified as edges, thereby facilitating the generation of an edge graph.

\subsection{Pristine and Forged Images}
In \Cref{fig:Visual_Full}, we presented synthetic images corresponding to four major conditions of DiFF, along with their synthesis process. Specifically, each forged image is generated using specific prompts and maintains semantic consistency with these prompts. All of these prompts are collected from facial features in real images, thus establishing an association between each synthetic image and the pristine images.

Subsequently, \Cref{fig:pristine} -- \Cref{fig:CycleDiff} showcase large collections of pristine and synthetic images in DiFF from different synthesized methods, respectively.

\begin{figure*}[t]
    \centering
    \includegraphics[width=0.98\textwidth]{sec/_Image/pristine.pdf}
    \caption{Visualization results of pristine images.}
    \label{fig:pristine}
\end{figure*}

\begin{figure*}[t]
    \centering
    \includegraphics[width=0.98\textwidth]{sec/_Image/Midjourney.pdf}
    \caption{Visualization results of Midjourney (T2I subset).}
    \label{fig:midjorney}
\end{figure*}

\begin{figure*}[t]
    \centering
    \includegraphics[width=0.98\textwidth]{sec/_Image/SDXL.pdf}
    \caption{Visualization results of SDXL (T2I subset).}
    \label{fig:SDXL}
\end{figure*}

\begin{figure*}[t]
    \centering
    \includegraphics[width=0.98\textwidth]{sec/_Image/FreeDom_T.pdf}
    \caption{Visualization results of FreeDom\_T (T2I subset).}
    \label{fig:FreeDomT}
\end{figure*}

\begin{figure*}[t]
    \centering
    \includegraphics[width=0.98\textwidth]{sec/_Image/HPS.pdf}
    \caption{Visualization results of HPS (T2I subset).}
    \label{fig:hps}
\end{figure*}

\begin{figure*}[t]
    \centering
    \includegraphics[width=0.98\textwidth]{sec/_Image/SDXL_Refiner.pdf}
    \caption{Visualization results of SDXL Refiner (I2I subset).}
    \label{fig:SDXL_Refiner}
\end{figure*}

\begin{figure*}[t]
    \centering
    \includegraphics[width=0.98\textwidth]{sec/_Image/LoRA.pdf}
    \caption{Visualization results of LoRA (I2I subset).}
    \label{fig:LoRA}
\end{figure*}

\begin{figure*}[t]
    \centering
    \includegraphics[width=0.98\textwidth]{sec/_Image/DreamBooth.pdf}
    \caption{Visualization results of DreamBooth (I2I subset).}
    \label{fig:DreamBooth}
\end{figure*}

\begin{figure*}[t]
    \centering
    \includegraphics[width=0.98\textwidth]{sec/_Image/FreeDoM_I.pdf}
    \caption{Visualization results of FreeDoM\_I (I2I subset).}
    \label{fig:FreeDoM_I}
\end{figure*}

\begin{figure*}[t]
    \centering
    \includegraphics[width=0.98\textwidth]{sec/_Image/DiffFace.pdf}
    \caption{Visualization results of DiffFace (FS subset).}
    \label{fig:DiffFace}
\end{figure*}

\begin{figure*}[t]
    \centering
    \includegraphics[width=0.98\textwidth]{sec/_Image/DCFace.pdf}
    \caption{Visualization results of DCFace (FS subset).}
    \label{fig:DCFace}
\end{figure*}

\begin{figure*}[t]
    \centering
    \includegraphics[width=0.98\textwidth]{sec/_Image/Imagic.pdf}
    \caption{Visualization results of Imagic (FE subset).}
    \label{fig:Imagic}
\end{figure*}

\begin{figure*}[t]
    \centering
    \includegraphics[width=0.98\textwidth]{sec/_Image/CoDiff.pdf}
    \caption{Visualization results of CoDiff (FE subset).}
    \label{fig:CoDiff}
\end{figure*}

\begin{figure*}[t]
    \centering
    \includegraphics[width=0.98\textwidth]{sec/_Image/CycleDiff.pdf}
    \caption{Visualization results of CycleDiff (FE subset).}
    \label{fig:CycleDiff}
\end{figure*}

% \begin{figure*}[t]
%     \centering
%     \includegraphics[width=0.95\textwidth]{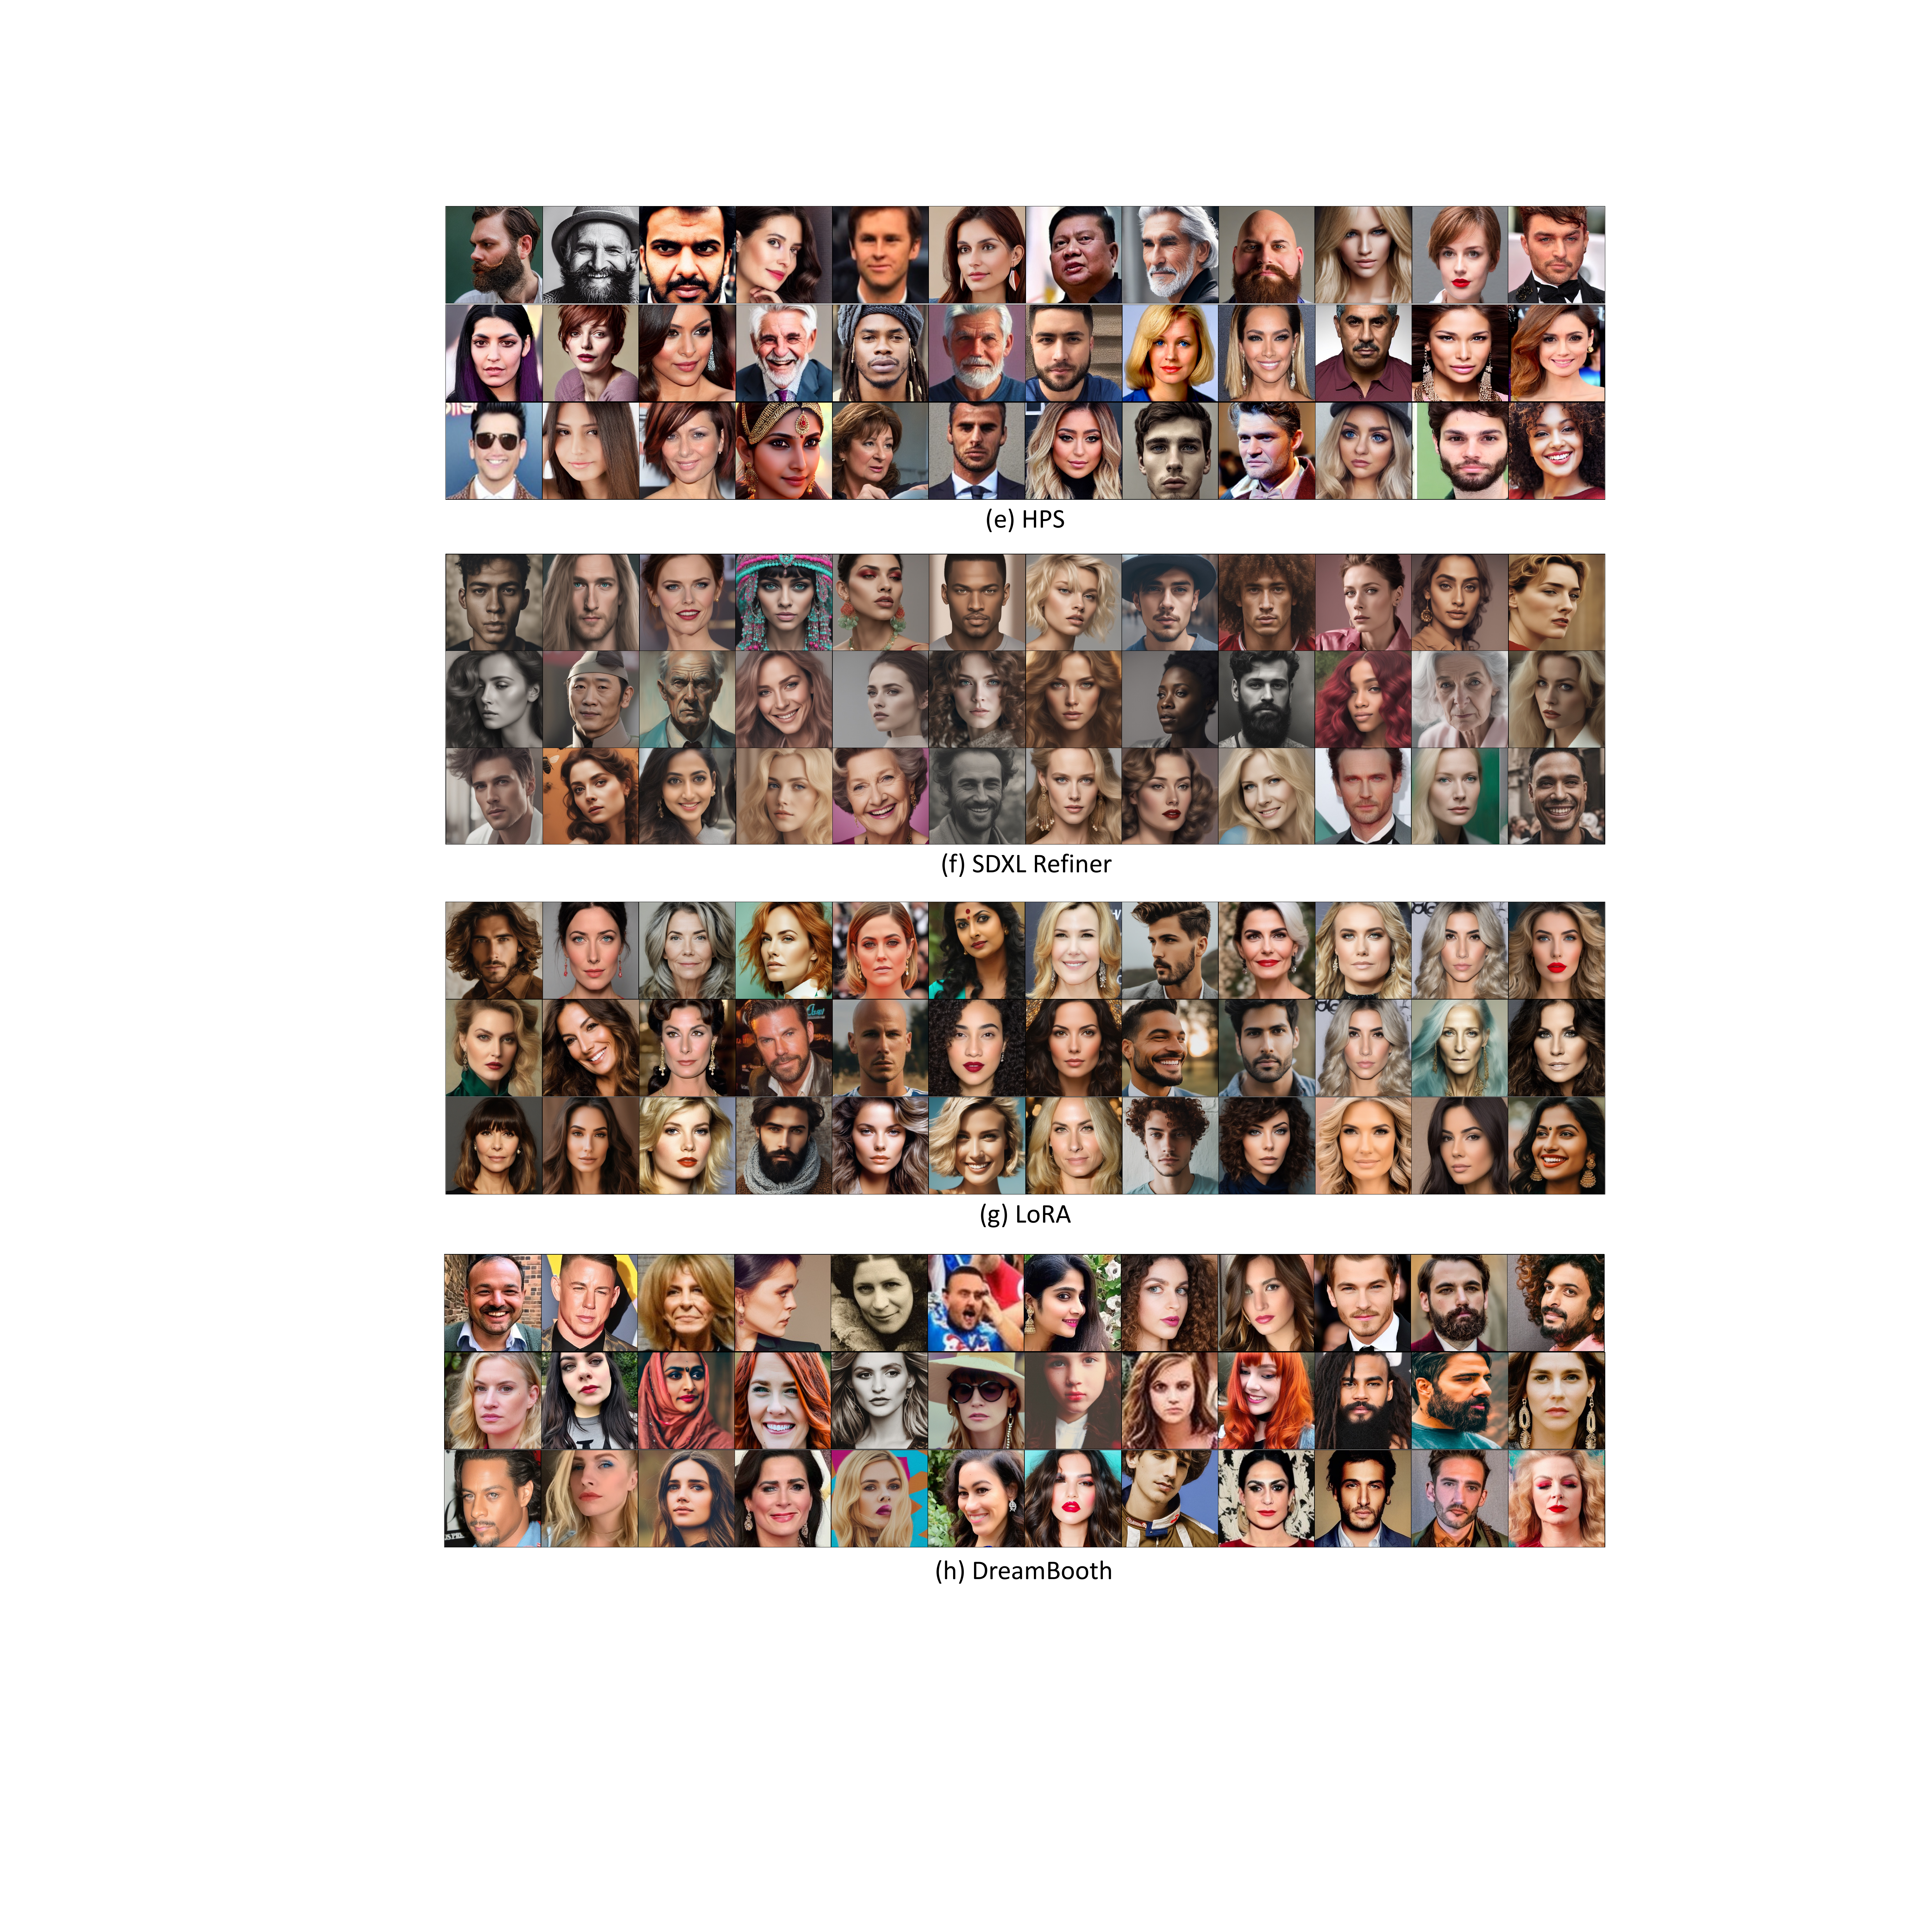}
%     \caption{Visualization results of DiFF.}
%     \label{fig:I2I}
% \end{figure*}

% \begin{figure*}[t]
%     \centering
%     \includegraphics[width=0.95\textwidth]{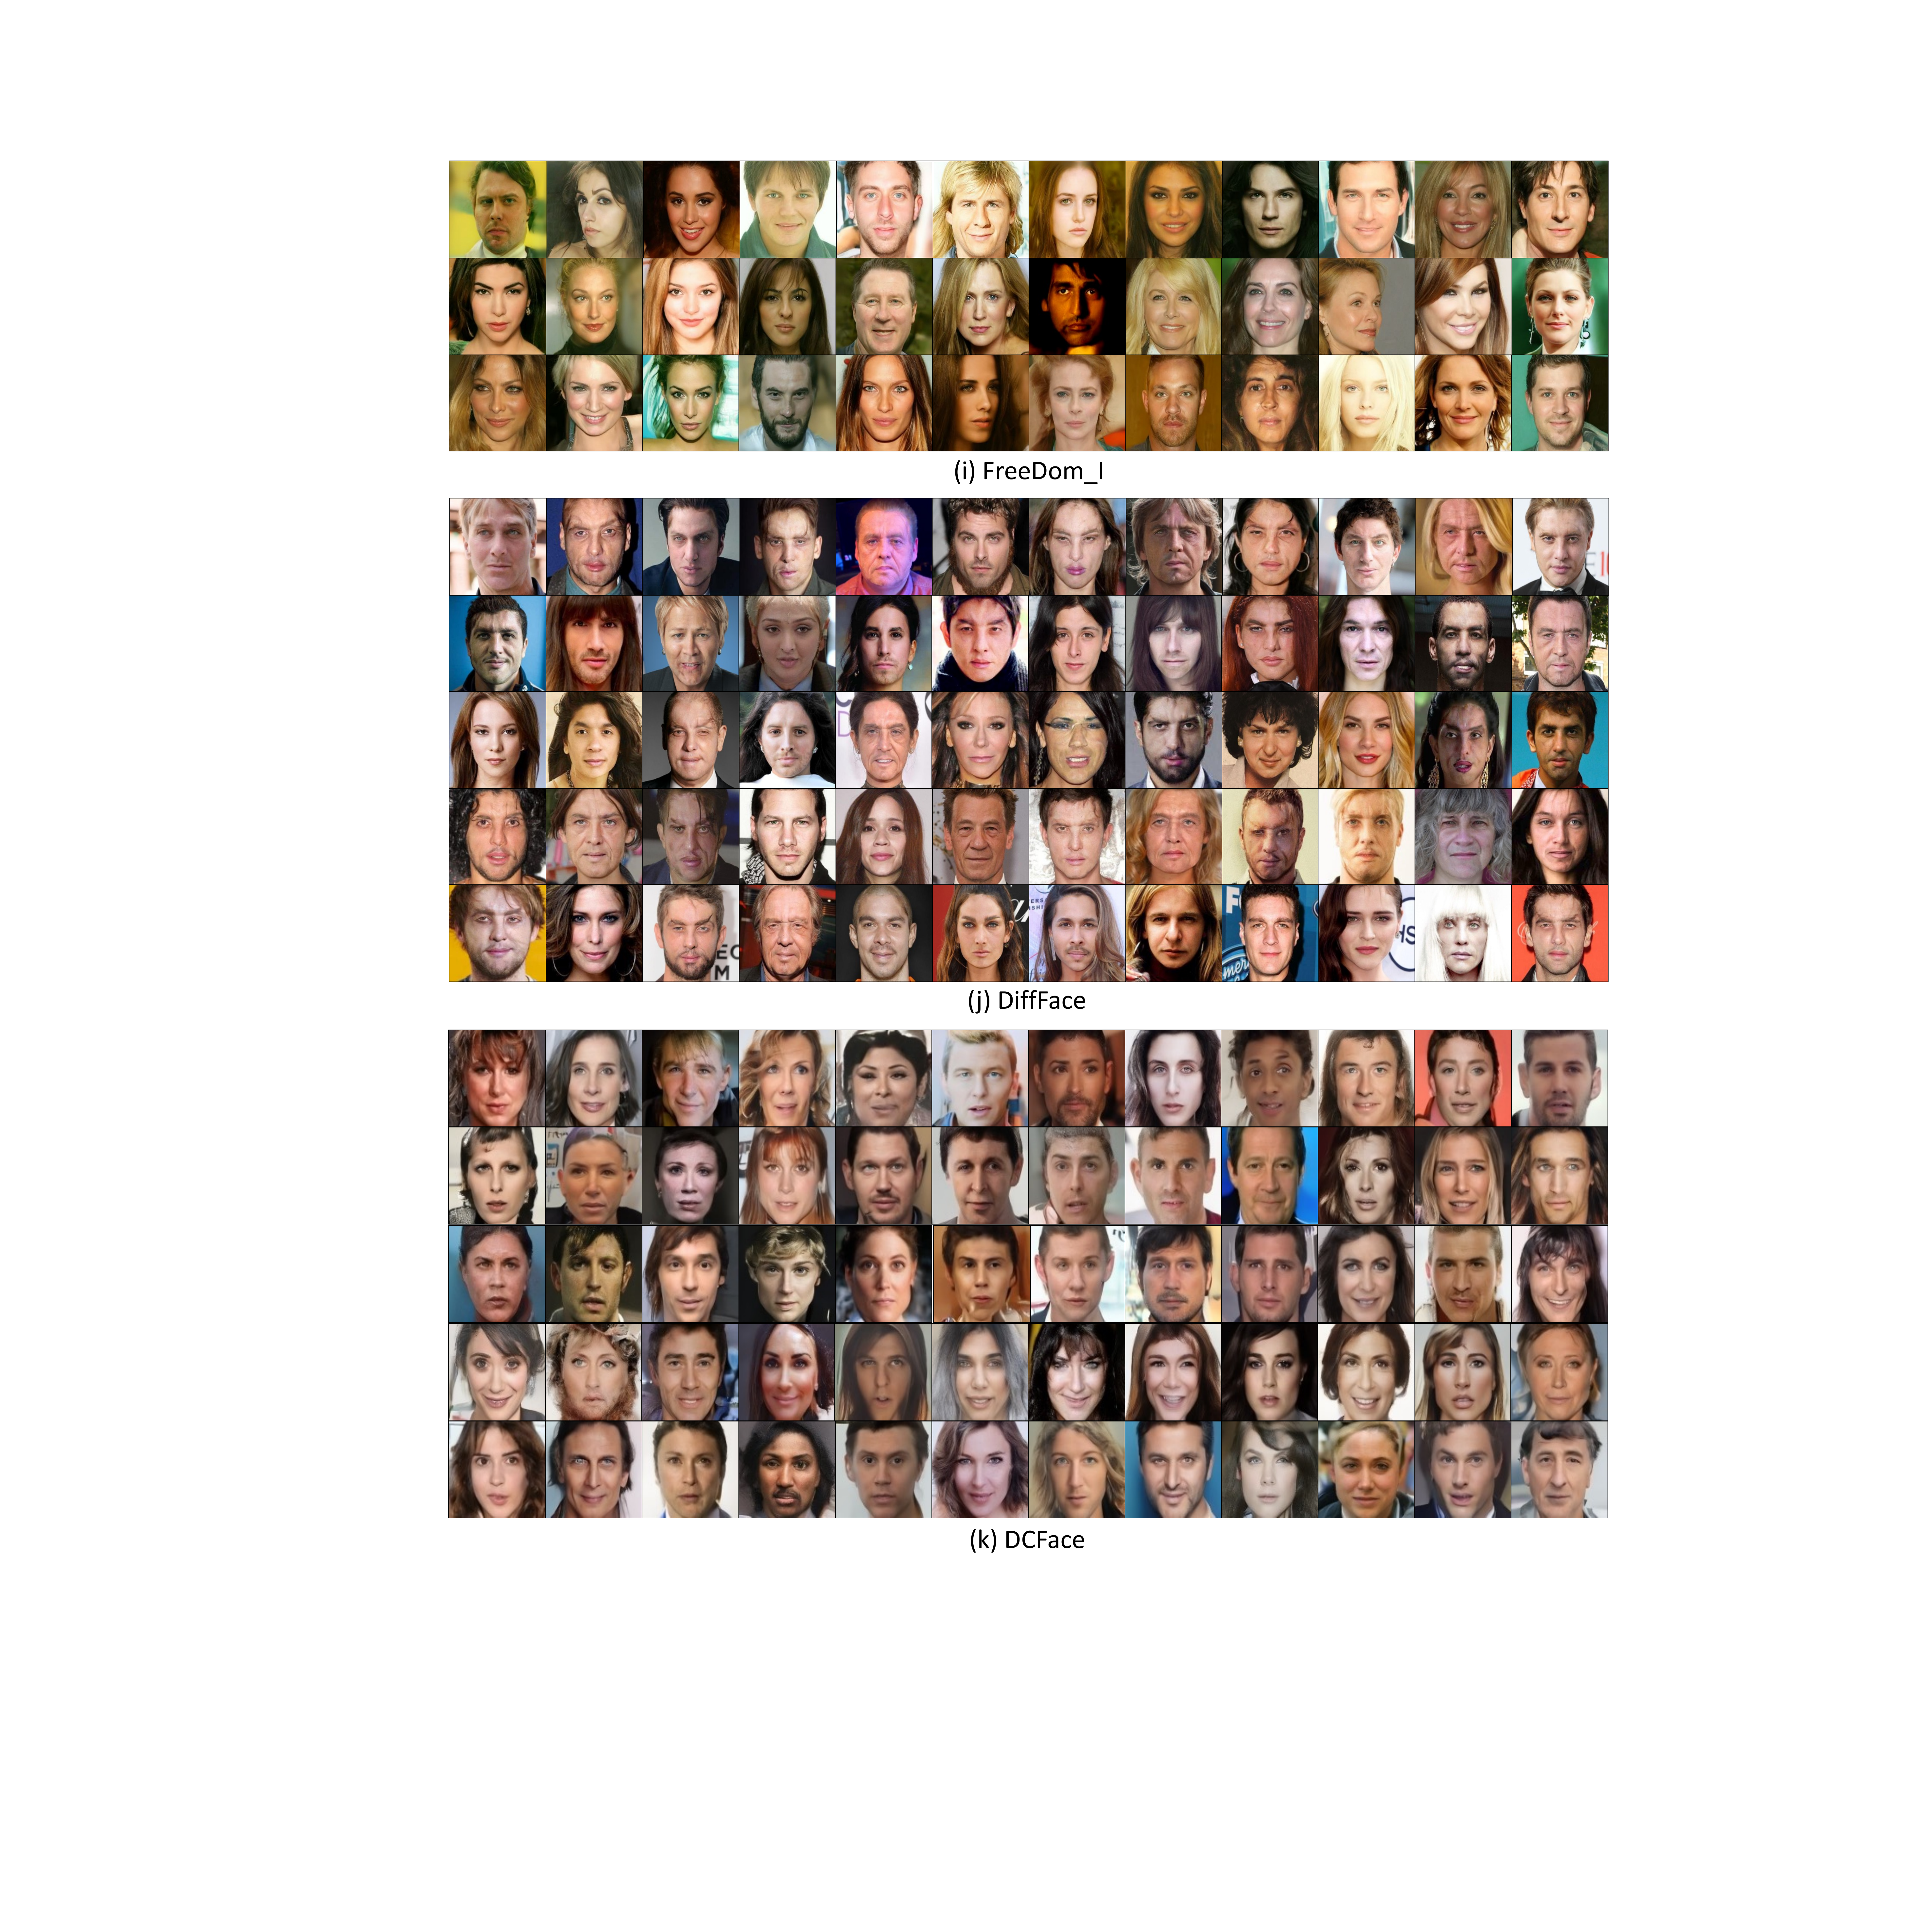}
%     \caption{Visualization results of DiFF.}
%     \label{fig:FS}
% \end{figure*}

% \begin{figure*}[t]
%     \centering
%     \includegraphics[width=0.95\textwidth]{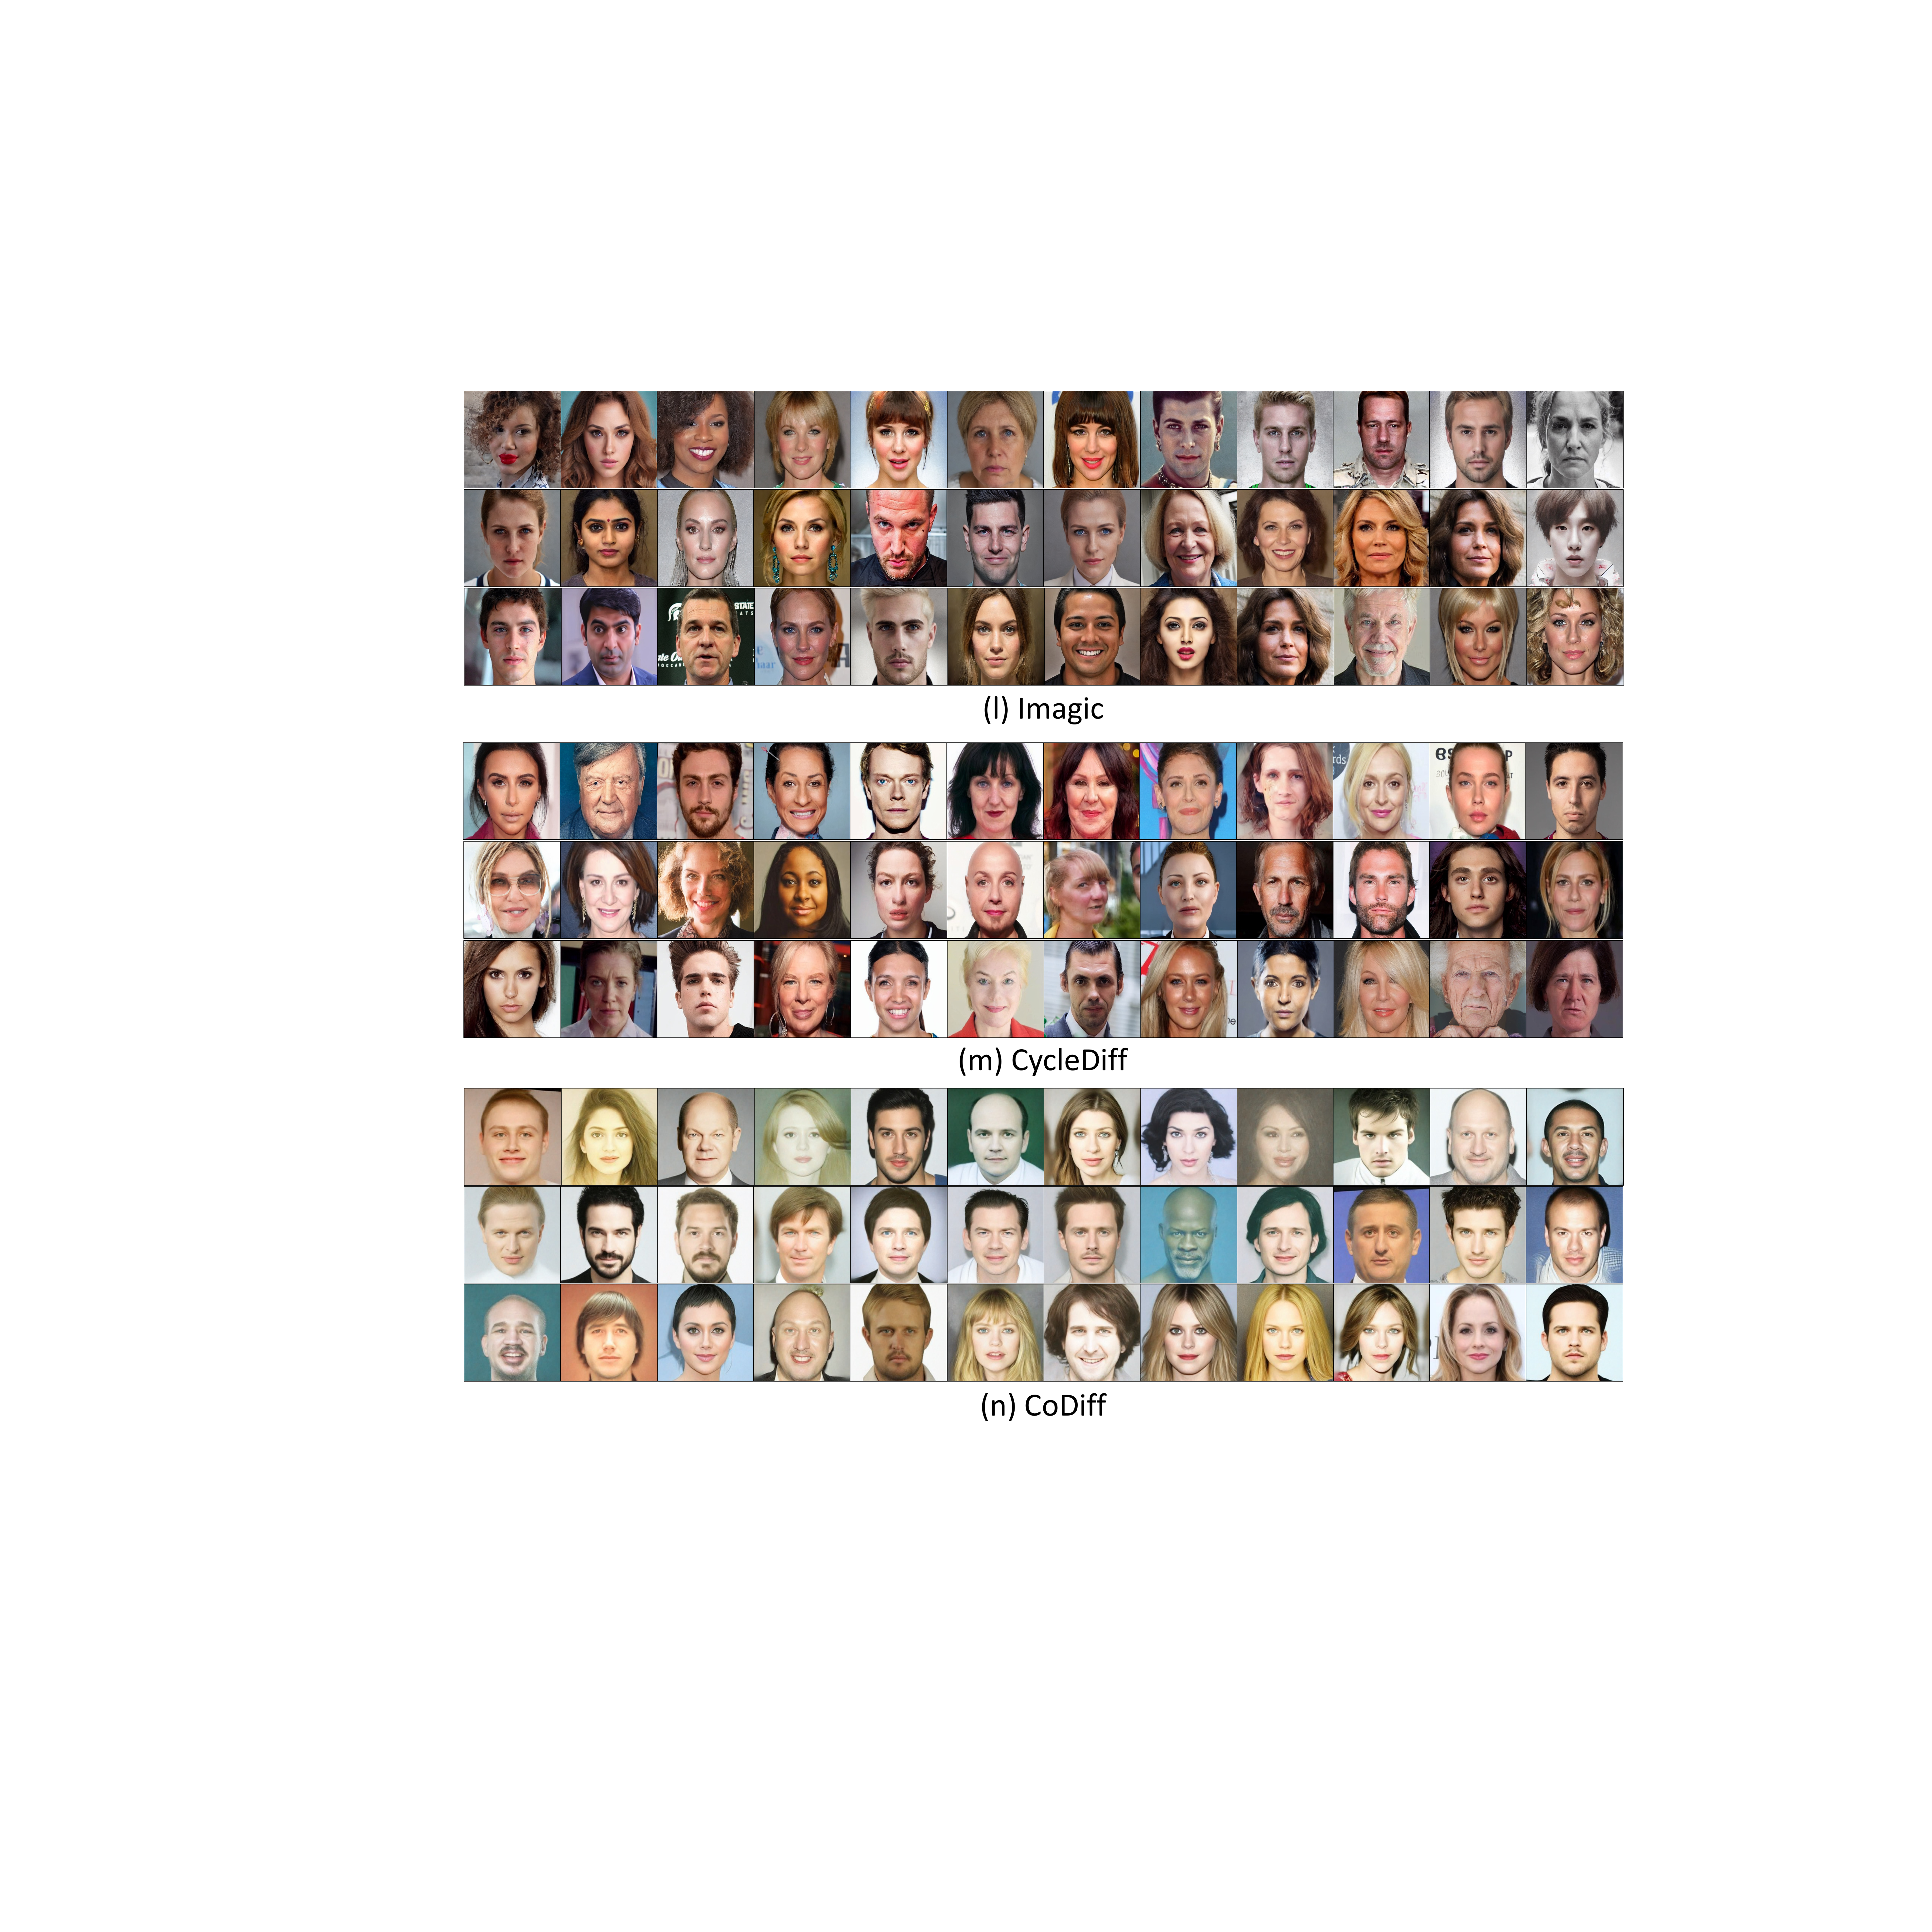}
%     \caption{Visualization results of DiFF.}
%     \label{fig:FE}
% \end{figure*}
